# Supplementary material for: Transfer Learning with General Estimating Equations
Source: arXiv:2410.04398 source file (2024-10-06)
Supplement: Supplementary file 1 [file appendix.tex]

\def\dphi{d_{\phi}}
\def\hdphi{\wh{d}_{\phi}}

\def\projr{\Pi_{\cF_N} \bar{r}_{\bv, \ell_2}(\wh{r}, \epsilon_N)}
\def\barr{\bar{r}_{\bv, \ell_2}(\wh{r}, \epsilon_N)}
\def\hetak{\wh{\bfeta}}

\iffalse
\begin{center}
\textbf{Organization}
\end{center}
\tableofcontents
\fi

\paragraph*{Notations}
Throughout the supplementary material, we use $c$ and $C$ with different subscripts to denote generic finite positive constants
that do not depend on $(p, n , m)$ and may be different in different uses. We use $\mathcal{N}(\delta; \mathcal{G},\norm{\cdot}_{\infty})$ to denote the cardinality of the smallest $\delta$-cover of the function class $\mathcal{G}$ with respect to the supremum norm for any $\delta > 0$. The empirical measure is denoted as $\E_{n}(\cdot)$.  

We will also use the following notations in the literature on empirical processes. Let $\pdim(F)$ be the the Pseudo dimension (\citealp{pollard1990}) of the function class $\mathcal{F}$. The $\varepsilon$-covering number of the function class $F$ with respect to the metric $d$ is denoted as $\mathcal{N}(\varepsilon, \mathcal{F}, d )$. For given $\bz_{1}^n = (\bz_{1}, \cdots, \bz_{n})$, we use $\mathcal{N}_{p}(\varepsilon, \mathcal{F}, \bz_{1}^n)$ to denote the $\varepsilon$-covering number of $\mathcal{F}$ with respect to $\norm{\cdot}_{L_{p}(\mu_{n})}$ norm for $p \in [1,\infty]$, where $\mu_{n}$ is empirical measure on $\bz_{1}^n$.

\section{ Proofs for Section 3}
\subsection{ Proof of Theorem 3.1}

In the sequel, we use $\E_0$ and $\E_{\tau}$  to denote the expectation under the true distribution $F$ and the regular parametric submodel $F_{\tau}$, respectively. 
The density function for $F_{\tau}$ is   
\begin{equation*}
	f_{\tau}(\bw) = p^\delta(1-p)^{1-\delta} f_{\tau}(\by|\bx)^{1-\delta} q_{\tau}(\bx)^\delta p_{\tau}(\bx)^{1-\delta},
\end{equation*} 
and the score function is given by 
\begin{equation*}
	S_{\tau}(\bw) = (1-\delta) S_{\tau}(\by|\bx) + \delta S_{\tau}^1 (\bx) + (1-\delta) S_{\tau}^0(\bx ),
\end{equation*}
where $S_{\tau}(\by | \bx) = \partial \log f_{\tau}(\by|\bx) / \partial \tau$, $S_{\tau}^0(\bx) = \partial \log p_{\tau}(\bx) / \partial \tau$ and  $S_{\tau}^1(\bx) = \partial \log q_{\tau}(\bx) / \partial \tau$,
satisfying 
\begin{equation}\label{eq: s1}
    \E_{\tau} \{ S_{\tau} (\bY | \bX) | \bX \} = \bzero, ~  \E_{\tau} \{ \delta S_{\tau}^1(\bX) \} = \bzero   ~\text{and}~ \E_{\tau} \{ (1-\delta)S_{\tau}^0(\bX) \} = \bzero.    
\end{equation}

\noindent \textbf{(i)} Since $\E_{\tau} \{ \bg\drw (\bW, \btheta, r(F_{\tau})) \} = 0$, differentiating with respect to $\tau$ gives 
\begin{equation}\label{eq: s2}
    \frac{\partial}{\partial \tau} \E_{\tau} \{ \bg\drw(\bW,\btheta, r(F_{\tau}))\}\Big\vert_{\tau = 0} =   \frac{\partial}{\partial \tau} \E_{\tau} \{ \bg\drw(\bW,\btheta, r_0)\}\Big\vert_{\tau = 0} +  \frac{\partial}{\partial \tau} \E_{0}\{ \bg\drw(\bW,\btheta, r(F_{\tau}))\}\Big\vert_{\tau = 0}. 
\end{equation} 
Under Condition 2 and the  mean-squared differentiability of the submodel $F_{\tau}$,  for any $\btheta \in \Theta_{0}$, the differentiation and integration operators are exchangeable (see, e.g., \citealp{ibragimov1981}) and it holds that 
\begin{equation}\label{eq: s3}
    \frac{\partial}{\partial \tau} \E_{\tau} \{ \bg\drw(\bW,\btheta, r_0)\}\Big\vert_{\tau = 0} 
    = \E_{0} \{ \bg\drw(\bW,\btheta, r_0) S_{0}(\bW)\}.  
\end{equation} 
We now calculate the right-hand side of \eqref{eq: s2}. By Lemma \ref{lem: s1}, 
\[
    \E_{\tau} \{ \bg\drw(\bW,\btheta, r(F_{\tau}))\} = \E_{\tau} \left\{ \frac{1-\delta}{1-p} \bg(\bZ, \btheta) r(F_{\tau}) \right\} = \E_{\tau} \left\{ \frac{\delta}{p} \bg(\bZ, \btheta) \right\}.  
\] 
Differentiating with respect to $\tau$ gives  
\begin{align}
    \frac{\partial}{\partial \tau} \E_{\tau} \{ \bg\drw(\bW,\btheta, r(F_{\tau}))\}\Big\vert_{\tau = 0} &=  \frac{\partial}{\partial \tau} \E_{\tau} \left\{ \frac{\delta}{p} \bg(\bZ, \btheta) \right\}\Big\vert_{\tau = 0} \nn \\ 
& =  \E_{0} \left\{ \frac{\delta}{p} \bg(\bZ, \btheta)S_{0}(\bW) \right\} \nn \\ 
& = \E_{0} \left\{ \frac{\delta}{p} \bg(\bZ, \btheta)S_{0}(\bX) +\frac{\delta}{p} \bg(\bZ, \btheta)S_{0}(\bY|\bX) \right\} \nn \\ 
& = \E_{0} \left\{ \frac{\delta}{p} \bbm_{0}(\bX, \btheta)S_{0}(\bW) \right\} + \E_{0} \left\{ \bg\drw(\bW, \btheta, r_{0})S_{0}(\bY | \bX)  \right\},  \label{eq: s4}
\end{align}
where the first term of \eqref{eq: s4} is from \eqref{eq: s1} and iterated expectation, and the second term is from Lemma \ref{lem: s1}.  We proceed to find a function $\bh(\bW)$ such that the second  term is equivalent to $\E_{0} \{ \bh(\bW)S_{0}(\bW) \}.$ Note that 
\begin{align}
     \E_{0} \left\{ \bg\drw(\bW, \btheta, r_{0})S_{0}(\bY | \bX)  \right\} 
    &=\E_{0} \left[   \bg\drw(\bW, \btheta, r_{0}) \{ S_{0}(\bW) - (1-\delta) S_{0}(\bX) \}   \right] \nn \\ 
    & =  \E_{0} \left\{ \bg\drw(\bW, \btheta, r_{0})S_{0}(\bW)  \right\} -  \E_{0} \left\{ \bg\drw(\bW, \btheta, r_{0})S_{0}(\bX)  \right\}, \nn  
\end{align}
and the second term is equivalent to 
\begin{align}\label{eq: s5}
    \E_{0} \left\{ \bg\drw(\bW, \btheta, r_{0})S_{0}(\bX)  \right\} = \E \left\{ \frac{1-\delta}{1-p} r_{0}(\bX) \bbm_{0}(\bX,\btheta) S_{0}(\bX) \right\} =   \E \left\{ \frac{1-\delta}{1-p} r_{0}(\bX) \bbm_{0}(\bX,\btheta) S_{0}(\bW) \right\}, 
\end{align}
where the first equality is by the iterated expectation, and the second equality is because of \eqref{eq: s1}. Combining \eqref{eq: s2}-\eqref{eq: s5} gives 
\begin{equation}
    \frac{\partial}{\partial \tau} \E_{0} \{ \bg\drw(\bW,\btheta, r(F_{\tau}))\}\Big\vert_{\tau = 0}=   \E_{0} \left\{ \bvphi(\bW, \btheta, \bfeta_{0})  S_{0}(\bW) \right\}, \nn
\end{equation}   
where $\bfeta_{0}(\bx) = (r_{0}(\bx), \bbm_{0}(\bx))$ and 
\begin{equation*}
    \bvphi(\bw, \btheta, \bfeta) = \frac{\delta}{p} \bbm(\bx, \btheta) - \frac{1-\delta}{1-p}{r}(\bx) \bbm(\bx, \btheta),
\end{equation*}
It is straightforward to see that $\E_{0} \{  \bvphi(\bw, \btheta, \bfeta_{0})  \} = \bzero$
for any $\btheta \in \bTheta_{0}$. In addition, because the set of score functions is dense in $L_{2}(F)$, the influence function $\bvphi$ is uniquely determined.   

\noindent \textbf{(ii)}
Let  $\bPsi(\bw, \btheta, \bfeta) =  \bg\drw(\bw, \btheta, r) +  \bvphi(\bw, \btheta, \bfeta)$. Since $\E_{0} \{  \bvphi(\bw, \btheta, \bfeta_{0})  \} = \bzero$, replacing $F$ by $F_{\tau}$ gives 
$\E_{\tau} \{  \bvphi(\bw, \btheta, \bfeta(F_\tau))  \} = \bzero$. Differentiating this identity with respect to $\tau = 0$ gives 
\begin{align}
    \bzero & =   \frac{\partial}{\partial \tau}\E_{\tau} \{  \bvphi(\bw, \btheta, \bfeta(F_\tau))  \}\Big\vert_{\tau = 0} \nn  \\ 
    & =  \frac{\partial}{\partial \tau} \E_{\tau}  \left\{ \bvphi(\bW, \btheta, \bfeta_{0}) \right\} +    \frac{\partial}{\partial \tau} \E_{0} \{  \bvphi(\bw, \btheta, \bfeta(F_\tau))\} \label{eq: s6}\\
    & =   \E_{0}\left\{ \bvphi(\bW, \btheta, \bfeta_{0})  S_{0}(\bW) \right\} + \frac{\partial}{\partial \tau} \E_{0} \{  \bvphi(\bw, \btheta, \bfeta(F_\tau))\} \nn \\ 
    & =     \frac{\partial}{\partial \tau} \E_{0} \{ \bg\drw(\bW,\btheta, r(F_{\tau}))\}\Big\vert_{\tau = 0}  + \frac{\partial}{\partial \tau} \E_{0} \{  \bvphi(\bw, \btheta, \bfeta(F_\tau))\}\Big\vert_{\tau = 0} \label{eq: s7} \\ 
    & = \frac{\partial}{\partial \tau} \E_{0} \{  \bPsi(\bW, \btheta, \bfeta(F_\tau))\}\Big\vert_{\tau = 0}, \nn 
\end{align}  
where \eqref{eq: s6} is from differentiation by parts and \eqref{eq: s7} is from the result in (i). 

\noindent \textbf{(iii)} 
First, $\bPsi$ can be rewritten as 
\begin{equation*}
    \bPsi(\bw, \btheta, \bfeta) = \frac{\delta}{p}\bg(\bz, \btheta) + \left\{\frac{1-\delta}{1-p}r(\bx) - \frac{\delta}{p}\right\} \{ \bg(\bz, \btheta)  - \bbm(\bx, \btheta)\}.   
\end{equation*} 
Because $\E_{F} \{ \delta \bg(\bZ, \btheta_{0}) \} = \bzero$, we have
\begin{align}
    \E_{F} \{ \bPsi(\bW, \btheta_{0}, \bfeta) \} & = \E_{F} \left[  \left\{\frac{1-\delta}{1-p}r(\bX) - \frac{\delta}{p}\right\} \{ \bg(\bz, \btheta)  - \bbm(\bX, \btheta)\} \right] \nn \\ 
    & = \E_{F}  \left[  \left\{\frac{1-\delta}{1-p}r(\bX) - \frac{\delta}{p}\right\} \{ \bbm_{0}(\bX, \btheta)  - \bbm(\bX, \btheta)\} \right] \nn,
\end{align}
implying that $  \E_{F} \{ \bPsi(\bW, \btheta_{0}, \bfeta) \} = \bzero$ if either $r(\bx) \stackrel{a.e.}{=} r_{0}(\bx)$ or $\bbm(\bx, \btheta_{0})\stackrel{a.e.}{=}\bbm_{0}(\bx, \btheta_{0})$.  

Let $\bDelta(\bx,\btheta) = \bbm_{0}(\bx, \btheta) - \bbm(\bx, \btheta) = (\Delta_{1},\dots, \Delta_{r})\t$. Since $\E_{F}[ \{ (1-p)^{-1}(1-\delta) r_{0}(\bX) - p^{-1}\delta \} \bDelta(\bX, \btheta)] = \bzero,$   we have
\begin{align}
    \left| \E_{F} \{ \Psi_{j}(\bW, \btheta_{0}, \bfeta) \} \right| & = \left| \E_{F} \left[  \left\{\frac{1-\delta}{1-p}r_{0}(\bX) - \frac{1-\delta}{1-p}r(\bX)\right\}\Delta_{j}(\bX,\btheta_{0})\right] \right| \nn \\ 
    & = \left|\E_{P} [\{ r_{0}(\bX) - r(\bX) \} \Delta_{j}(\bX,\btheta_{0}) ]\right| \nn \\ 
    & \leq \E_{P} \{ |r_{0}(\bX) - r(\bX)| |\Delta_{j}(\bX,\btheta_{0})| \} \nn \\ 
    & \leq \norm{r - r_{0}}_{L_{2}(P_{X})}\norm{m_{j}(\cdot,\btheta_{0}) - m_{0j}(\cdot,\btheta_{0})}_{L_{2}(P_{X})}, \label{eq: s8}
\end{align}
which completes the proof.  \qed

\section{ Additional discussions on divergence functions}

\subsection{ Common $f$-divergences and their conjugates}

We summarize commonly used $f$-divergences' generator functions and their corresponding derivative functions and Fenchel conjugate functions below.   

\begin{table}[ht]
    \centering
    \caption{List of some popular $f$-divergences together with their generator functions, Fenchel conjugate functions  of generator functions, as well as the domain of the conjugate functions.}
    \begin{tabular}{c c c c c}
    \hline
        Divergence &  $\phi(u)$ & $\phi'(u)$ &  $ \phi_{*}(v)$ & $\rm{dom}( \phi_{*})$ \\
    \hline 
        Kullback-Leibler & $ u \log(u)$ & $\log(u) + 1$ & $\exp(v -1)$ & $\mathbb{R}$   \\ 
        Reverse KL &  $-\log(u)$ & $-\frac{1}{u}$ & $-1 - \log(-v)$ & $\mathbb{R}_{-} $  \\
        Pearson $\chi^2$ & $(u-1)^2$ & $2(u-1)$ &  $\frac{1}{4}v^2 + v$ & $\mathbb{R} $  \\ 
        Neyman $\chi^2$ & $\frac{1}{u} - 1$ & $-\frac{1}{u^2}$  & $-2 \sqrt{-v} - 1$  & $\mathbb{R}_{-} $   \\ 
        Squared Hellinger & $(\sqrt{u}-1)^2$  & $1 - \frac{1}{\sqrt{u}}$ & $\frac{v}{v-1}$ &  $(-\infty,1)$  \\  
    \hline 
    \end{tabular}
    \label{tab: divergence}
\end{table}

\subsection{ Criterion functions for density ratio estimation}
\label{sec: cri-dre}
Recall that for any $\phi$ with the conjugate $\phi_{*}$, the variational characterization of the $f$-divergence proposed by \cite{nguyen2010} with the generator $\phi$ is represented by
\begin{equation}
    D_{\phi}(Q \| P) \geq \sup_{f \in \mathcal{F} }\left\{ \E_Q (f)  - \E_P\left( \phi_{*}(f)\right) \right\}% =: \sup_{f \in \mathcal{F} } \E_{F} L(f),
    \nn 
\end{equation}
%with 
%\begin{align}
%    L(f) = \frac{\delta}{p} f - \frac{1-\delta}{1-p} \phi_{*}(f)
%\end{align} 
and the supreme is attained at $f_{0}(\bx) = \phi'\left( \frac{q_0(\bx)}{p_0(\bx)}\right) = \phi'\left( r_0(\bx) \right)$, if it is contained in $\mathcal{F}$, where $\mathcal{F}$ should be defined on $\text{dom}(\phi_{*})$. 
Therefore, the density ratio function $r_{0}$ satisfies 
\begin{align}
    r_{0} = (\phi')^{-1}(f_{0}), ~~\text{where}~ f_{0} = \argmin_{f \in \mathcal{F}}\E_{F} \left\{\frac{1-\delta}{1-p} \phi_{*}(f) - \frac{\delta}{p} f \right\}
\end{align}

We now present the criterion functions for density ratio function estimation under different specifications of $f$-divergences listed in \cref{tab: divergence}.

\noindent 1.  Kullback-Leibler: since $\phi_{*}(v) = \exp(v -1)$, we define  
$$\tilde{\ell}(\bw, f) = \frac{1-\delta}{1-p} \exp(f(\bx) - 1) - \frac{\delta}{p}f(\bx), $$
where $f: \mathcal{X} \to \mathbb{R}$. 
The density ratio function satisfies 
\[
r_{0} = (\phi')^{-1}(f_{0})= \exp( f_{0} - 1 ),~~\text{where}~ f_{0} = \argmin_{f \in \mathcal{F}}\E_{F}  \tilde{\ell}(\bW, f).  
\] 
Letting $h = f+ 1$ and $h_{0} = f_{0} + 1$, then we have 
\begin{equation}
\begin{aligned}
    & r_{0} =\exp( h_{0} ),~~\text{where}~ h_{0} = \argmin_{h \in \mathcal{F}}\E_{F}  \ell(\bW, h)   \\ 
    \text{and}~~  & \ell(\bw, h) = \frac{1-\delta}{1-p} \exp(h(\bx)) - \frac{\delta}{p}h(\bx).
\end{aligned}
\label{eq: KL}
\end{equation}

\noindent 2. Reverse KL: since $\phi_{*}(v) = -1- \log(-v)$, we define  
$$\tilde{\ell}(\bw, f) = \frac{1-\delta}{1-p} \left\{-1-\log(-f(\bx))  \right\}- \frac{\delta}{p}f(\bx), $$
where  $f: \mathcal{X} \to  \mathbb{R}_{-}$. 
The density ratio function satisfies 
\[
r_{0} = (\phi')^{-1}(f_{0})= - f_{0}^{-1},~~\text{where}~ f_{0} = \argmin_{f \in \mathcal{F}}\E_{F}  \tilde{\ell}(\bW, f).  
\]  
Letting $h = \log(- f)$ and $h_{0} = \log(- f_{0})$, then direct calculations show that 
\begin{equation}
    \begin{aligned}
    & r_{0} =  h_{0}^{-1},~~\text{where}~ h_{0} = \argmin_{h \in \mathcal{F}}\E_{F}  \ell(\bW, h) \\ 
  \text{and}~~  & \ell(\bw, h) = - \frac{1-\delta}{1-p} h(\bx) + \frac{\delta}{p}\exp(h(\bx)).  
\end{aligned}
\label{eq: reverse KL-1}
\end{equation}
Because $h_{0} = p_{0} / r_{0}$, which is the inverse of our target density ratio. To aviod taking $r_{0} = h_{0}^{-1}$, we switch the roles of two samples in \eqref{eq: neyman-s1} and obtain: 
\begin{equation}
    \begin{aligned}
    & r_{0} =  h_{0},~~\text{where}~ h_{0} = \argmin_{h \in \mathcal{F}}\E_{F}  \ell(\bW, h) \\ 
  \text{and}~~  & \ell(\bw, h) = - \frac{\delta}{p} h(\bx) + \frac{1-\delta}{1-p} \exp(h(\bx)),
\end{aligned}
\label{eq: reverse KL-2}
\end{equation}
which is equivalent to the criterion function \eqref{eq: KL} with the KL-divergence.

\noindent 3. Pearson $\chi^2$: since $\phi_{*}(v)= \frac{1}{4}v^2 + v$, we define 
\[
    \tilde{\ell}(\bw, f) = \frac{1-\delta}{1-p}\left(\frac{1}{4}f^2(\bx) + f(\bx)\right) - \frac{\delta}{p} f(\bx),
\]   
where  $f: \mathcal{X} \to  \mathbb{R}$.  The density ratio function satisfies 
\[
    r_{0} = (\phi')^{-1}(f_{0})= \frac{f_{0}}{2} + 1, ~~\text{where}~ f_{0} = \argmin_{f \in \mathcal{F}}\E_{F}  \tilde{\ell}(\bW, f).  
\] 
Letting $h = \frac{f}{2} + 1$ and $h_{0} = \frac{f_{0}}{2} + 1$, then direct calculations show that 
\begin{equation}
    \begin{aligned}
    & r_{0} =  h_{0},~~\text{where}~ h_{0} = \argmin_{h \in \mathcal{F}}\E_{F}  \ell(\bW, h) \\ 
  \text{and}~~  & \ell(\bw, h) =  \frac{1-\delta}{1-p} (\left(h^2(\bx) + h(\bx) \right) - 2\frac{\delta}{p} h(\bx).  
\end{aligned}
\end{equation}

\noindent 4. Neyman $\chi^2$: since $\phi_{*}(v)= -2\sqrt{-v}-1$, we define 
\[
    \tilde{\ell}(\bw, f) = -2\frac{1-\delta}{1-p}\sqrt{-f(\bx)} - \frac{\delta}{p} f(\bx),
\]   
where  $f: \mathcal{X} \to  \mathbb{R}_{-}$.  The density ratio function satisfies 
\[
    r_{0} = (\phi')^{-1}(f_{0})= \sqrt{-\frac{1}{f_{0}}}, ~~\text{where}~ f_{0} = \argmin_{f \in \mathcal{F}}\E_{F}  \tilde{\ell}(\bW, f).  
\] 
Letting $h = \sqrt{-f}$ and $h_{0} =  \sqrt{-f_{0}}$, then direct calculations show that 
\begin{equation}
    \begin{aligned}
    & r_{0} =  h_{0}^{-1},~~\text{where}~ h_{0} = \argmin_{h \in \mathcal{F}}\E_{F}  \ell(\bW, h) \\ 
  \text{and}~~  & \ell(\bw, h) =  -2\frac{1-\delta}{1-p} h(\bx) + \frac{\delta}{p} h^2(\bx).  
\end{aligned}
\label{eq: neyman-s1}
\end{equation}
Because $h_{0} = p_{0} / r_{0}$, which is the inverse of our target density ratio. To aviod taking $r_{0} = h_{0}^{-1}$, we switch the roles of two samples in \eqref{eq: neyman-s1} and obtain: 
\begin{equation}
    \begin{aligned}
    & r_{0} =  h_{0},~~\text{where}~ h_{0} = \argmin_{h \in \mathcal{F}}\E_{F}  \ell(\bW, h) \\ 
  \text{and}~~  & \ell(\bw, h) =  \frac{1-\delta}{1-p} h^2(\bx)  -2\frac{\delta}{p} h(\bx).  
\end{aligned}
\label{eq: neyman-2}
\end{equation}

\noindent 5. Squared Hellinger: since $\phi_{*}(v) = 1+ \frac{1}{v-1}$, we define 
\[
    \tilde{\ell}(\bw, f) = \frac{1-\delta}{1-p} \left(1+ \frac{1}{f(\bx) -1 }\right) - \frac{\delta}{p}f(\bx),
\]  
where $f: \mathcal{X} \to (-\infty, 1)$. 
The density ratio function satisfies 
\[
r_{0} = (\phi')^{-1}(f_{0})= \left(\frac{1}{f_{0}-1}\right)^2 ,~~\text{where}~ f_{0} = \argmin_{f \in \mathcal{F}}\E_{F}  \tilde{\ell}(\bW, f).  
\]  
Letting $h = \frac{1}{1-f}$ and $h_{0} = \frac{1}{1-f_{0}}$, we have
\begin{equation}
    \begin{aligned}
    & r_{0} =  h_{0}^{2},~~\text{where}~ h_{0} = \argmin_{h \in \mathcal{F}}\E_{F}  \ell(\bW, h) \\ 
  \text{and}~~  & \ell(\bw, h) = - \frac{1-\delta}{1-p} h(\bx) + \frac{\delta}{p}\frac{1}{h}.  
\end{aligned}
\end{equation}

\section{ Proofs for Section \ref{sec: m2}}
\label{sec: proof for dre}

\subsection{ Proof of Theorem \ref{thm3}} 
%To simplify notation, we conduct the proof under the full-sample setting where all observations in $\mathcal{D}_0$ and $\mathcal{D}_1$ are used for estimating the target function $r_0$, since the result of the cross-fitting version can be directly extended to. 
Our proof proceeds in several steps. In Step 1, we present an error decomposition for $\norm{\widehat{r} - r_{0}}^2_{L_{2}(P)}$. In Steps 2 - 4, we investigate the deviations between the sample and population excess risks via empirical process theories. 

\ni {\bf Step 1: Error decomposition.} 
Denote $\ell_{1}(r, \bx) = \phi_{*}\left\{\phi'(\bx)\right\}, \ell_{2}(r, \bx) = -\phi'(\bx)$. Let $\mathcal{L}_{1}(r) = \E_{P}\left\{ \ell_{1}(r, \bX)\right\}$, $\mathcal{L}_{2}(r) = \E_{Q}\left\{ \ell_{2}(r, \bX)\right\}$, and $\widehat{\mathcal{L}}_{1}(r) = n^{-1}\sum_{i=1}^n\ell_{1}(r, \bX_{i})$, $\widehat{\mathcal{L}}_{2}(r) = m^{-1}\sum_{i=n+1}^{n+m}\ell_{2}(r, \bX_{i})$.   
The population and  the sample criterion function are: 
\[
\mathcal{L}(r) := \mathcal{L}_{1}(r) + \mathcal{L}_{1}(r)  ~~\text{ and }~~
\widehat{\mathcal{L}}(r) := \widehat{\cL}_{1}(r)  + \widehat{\cL}_{2}(r) .
\] 
For any $r_{1}, r_{2}: \mathcal{X} \to [0, \infty)$, let   
\[
    \dphi(r_{1}, r_{2}) := \mathcal{L}_{\phi}(r_{1}) - \mathcal{L}_{\phi}(r_{2}) ~~\text{ and }~~
\hdphi(r_{1}, r_{2}) = \widehat{\mathcal{L}}_{\phi}(r_{1}) - \widehat{\mathcal{L}}_{\phi}(r_{2}).
\] 
%where the former is the so-called excess risk, which is no less than zero for $r \in \mathcal{R}_{N}$, and the later is minimized at $\widehat{r}$ and $\widehat{d}_{\phi}(\widehat{r}, r_{0}) \leq 0$.    
%Our candidate function class is the non-negative ReLU-network class $\mathcal{R}_{N} = \mathcal{F}(L_{N}, W_{N}, d, 2B)$, where $d$ is the dimension of $\bX$ and $L_{N}$ and $W_{N}$ are the depth and the width, respectively, that remains to be determined later.       
Given a function class $\cF_N$, we define the best approximation for $r_{0}$ realized by $\cF_N$ and the corresponding approximation error as: 
\[
r_{N} := \argmin_{r \in \cF_N } \norm{r - r_{0}}_{\infty}~~~\text{and}~~~ \varepsilon_{N} := \norm{r_{N} - r_{0}}_{\infty}.
\]  
Note that $r_{N}$ and $\varepsilon_{N}$ are both deterministic and depend only on the architecture of $\cF_N$ and the target function $r_{0}$.      
By the definition of $\dphi$, % and Condition \ref{con: phi} (ii),
we have the following error decomposition: 
\iffalse
\begin{align}
    c_{1} \norm{\widehat{r} - r_{0}}^2_{L_{2}(P)}\leq & d_{\phi}\left(\widehat{r}, r_{0}\right) \nn \\
    \leq &  d_{\phi}\left(\widehat{r}, r_{0}\right) - \widehat{d}_{\phi}\left(\widehat{r}, r_{0}\right) + \widehat{d}_{\phi}\left( r_{N}, r_{0}\right) \nn \\
    \leq & \left\{   d_{\phi}\left(\widehat{r}, r_{0}\right) - \widehat{d}_{\phi}\left(\widehat{r}, r_{0}\right) \right\} + \left\{ \widehat{d}_{\phi}\left( r_{N}, r_{0}\right) - {d}_{\phi}\left( r_{N}, r_{0}\right) \right\} + {d}_{\phi}\left( r_{N}, r_{0}\right) \nn \\ 
    \leq & \left\{   d_{\phi}\left(\widehat{r}, r_{0}\right) - \widehat{d}_{\phi}\left(\widehat{r}, r_{0}\right) \right\} + \left\{ \widehat{d}_{\phi}\left( r_{N}, r_{0}\right) - {d}_{\phi}\left( r_{N}, r_{0}\right) \right\} + c_{2} \varepsilon_{N}^2. 
    \label{eq: error decom of r}
\end{align}
\fi 
\begin{align}
    c_{1} \norm{\widehat{r} - r_{0}}^2_{L_{2}(P)}\leq & d_{\phi}\left(\widehat{r}, r_{0}\right)= d_{\phi}\left(\widehat{r}, r_{N}\right) + d_{\phi}\left(r_{N}, r_{0}\right) \leq d_{\phi}\left(\widehat{r}, r_{N}\right) +  c_{2} \varepsilon_{N}^2. 
    %\nn \\ 
    %\leq & d_{\phi}\left(\widehat{r}, r_{N}\right) -  \widehat{d}_{\phi}\left(\widehat{r}, r_{N}\right)  + d_{\phi}\left(r_{N}, r_{0}\right) \nn \\ 
    %\leq & d_{\phi}\left(\widehat{r}, r_{N}\right) -  \widehat{d}_{\phi}\left(\widehat{r}, r_{N}\right)   + c_{2} \varepsilon_{N}^2. 
    \label{eq: hat-r-decom}
\end{align}

We next bound $\dphi\left(\widehat{r}, r_{N}\right)$ by analyzing the process $\sup_{r \in \mathcal{R}_{N} } |d_{\phi}\left({r}, r_{N}\right) -  \widehat{d}_{\phi}\left({r}, r_{N}\right)|$, mainly based on techniques of the local Rademacher complexity analysis of empirical risk minimization (\citealp{Bartlett2005} and \citealp{koltchinskii2011}). 
First, we introduce some quantities that are necessary in this approach.  
Let  $\{\varepsilon_{i}\}_{i=1}^{n+m}$ be i.i.d symmetric, $\left\{ -1,1\right\}$-valued random variables that are independent of $\left\{ \bX_{i}\right\}_{i=1}^{n+m}$. For any function class $\mathcal{F}$, we define 
\[
\cR_{n}(\mathcal{F} ) := \sup_{f \in \mathcal{F}} \frac{1}{n} \sum_{i=1}^n \varepsilon_{i} f(\bX_{i}), ~~~\cR_{m}(\mathcal{F} ) := \sup_{f \in \mathcal{F}} \frac{1}{m} \sum_{i=n+1}^{n+m} \varepsilon_{i} f(\bX_{i}). 
\]  
The Rademacher complexities are defined as $\widebar{\mathcal{R}}_{n}(\mathcal{F}) = \E \left\{ \cR_{n}(\mathcal{F} )\right\} $ and $\widebar{\mathcal{R}}_{m}(\mathcal{F}) = \E \left\{ \cR_{m}(\mathcal{F} )\right\}$, where the expectations are taken over both the $\bX_i$s and the  $\varepsilon_{i}$s. The empirical Rademacher complexities, which are conditioned on the data, are denoted by $\widehat{R}_{n}(\mathcal{F}) = \E_{\varepsilon}  \left\{ R_{n}(\mathcal{F} )\right\}$ and   $\widehat{R}_{m}(\mathcal{F}) = \E_{\varepsilon}  \left\{ R_{m}(\mathcal{F} )\right\}$. For the candidate function class $\cF_N$, let the shifted (centered) function class be 
\[
\mathcal{F}^*_{N} := \left\{ r - r_{N}: r \in \cF_N \right\}.  
\] 
The population version of the localized Rademacher complexities are defined as: 
\begin{align}
    \wb\cR_n(\delta, \mathcal{F}^*_{N} ) :=% \E_{\bX, \varepsilon} \left\{ 
   % \sup_{\substack{ f \in \mathcal{F}^*_{N}, d_{\phi}(f) \leq \delta^2 }} \abs{ \frac{1}{n} \sum_{i=1}^n \varepsilon_{i} f(\bX_{i})}\right\}, 
   \wb\cR_{n}\left\{f: f \in \mathcal{F}_{N}^*~ \text{and}~ \norm{f}_{L_{2}(P)} \leq \delta\right\}~~\text{and}~~    \widebar{\mathcal{R}}_{m}(\delta, \mathcal{F}^*_{N} ) :=\widebar{\mathcal{R}}_{m}\left\{f: f \in \mathcal{F}_{N}^*~ \text{and}~  \norm{f}_{L_{2}(Q)} \leq \delta \right\},
\nn 
\end{align} 
where $\delta > 0$ is a localization scale. Similarly, the empirical localized Rademacher complexities are defined as: 
\begin{align}
    \widehat{\mathcal{R}}_{n}(\delta, \mathcal{F}^*_{N} ) :=% \E_{\bX, \varepsilon} \left\{ 
   % \sup_{\substack{ f \in \mathcal{F}^*_{N}, d_{\phi}(f) \leq \delta^2 }} \abs{ \frac{1}{n} \sum_{i=1}^n \varepsilon_{i} f(\bX_{i})}\right\}, 
   \widehat{\mathcal{R}}_{n}\left\{f: f \in \mathcal{F}_{N}^*~ \text{and}~ \norm{f}_{n} \leq \delta \right\}~~\text{and}~~    \widehat{\mathcal{R}}_{m}(\delta, \mathcal{F}^*_{N} ) :=\widehat{\mathcal{R}}_{m}\left\{f: f \in \mathcal{F}_{N}^*~ \text{and}~ \norm{f}_{m} \leq \delta\right\}.
\nn 
\end{align} 
A crucial parameter in the localized Rademacher complexity approach is the critical radius, which is defined as $\delta_n$ and $\delta_m$ that satisfy the following inequalities: 
\begin{align}
    \delta_{n}^2 \geq  \widebar{\mathcal{R}}_{n}(\delta_{n}, \mathcal{F}^*_{N} ), ~~~  \delta_{m}^2 \geq  \widebar{\mathcal{R}}_{m}(\delta_{m}, \mathcal{F}^*_{N} ).  \label{eq: critical radius} 
\end{align} 
{For $j = 1$ and $2$, denote the supreme deviations between  
$\widehat{\mathcal{L}}_{j}(r) - \widehat{\mathcal{L}}_{j}(r_{0})$ 
and $\mathcal{L}_{j}(r) -  {\mathcal{L}}_{j}(r_{0})$ restricted in the localized ball centered at $r_{0}$ with the radius $s$ as  
\begin{align}
    \lambda_{N}^j(s) =  \sup_{\norm{r- r_{N}}_{L_{2}(P)} \leq s}\abs{ 
      \left( \widehat{\mathcal{L}}_{j}(r) - \widehat{\mathcal{L}}_{j}(r_{N}) \right)  -  \left(\mathcal{L}_{j}(r) -  {\mathcal{L}}_{j}(r_{N})\right),
    }
\end{align}
and denote  the supreme deviations between  $d_{\phi}(r, r_{N})$ and $\widehat{d}_{\phi}(r, r_{N})$ restricted in $d_{\phi}(r, r_{N})$ as  
\begin{align}
    \lambda_{N}(s) = \sup_{\norm{r- r_{N}}_{L_{2}(P)} \leq s} \abs{\widehat{d}_{\phi}(r, r_{N}) - d_{\phi}(r, r_{N}) },
\label{eq: lambda_N(s)}
\end{align}
where $s > 0$ is a radius to be varied.}

\bigskip

\ni {\bf Step 2. Tail bound of $\lambda_{N}(s)$ . }
We first estimate an upper bound of the expectation of $\lambda_{N}(s)$ for the $s$ in the range $[\delta_{n} \vee \delta_{m}, \infty)$. Let 
$$\mathcal{G}_{N}^j(s) = \left\{g: g =  \ell_{j}(r) -\ell_{j}(r_{0}) ~~\text{for}~ r \in \mathcal{R}_{N}~\text{and}~    \dphi(r, r_{0}) \leq s^2  \right\} $$ 
%and $$ 
%%\mathcal{G}_{N}^2(s) = \left\{g: g =  \phi'(r) -\phi'(r_{0}) ~~\text{with}~ r \in \mathcal{R}_{N}~\text{and}~    d(r, r_{0}) \leq s^2  \right\}.  
%$$
for $j = 1$ and $2$.  
Then by standard symmetrization arguments, we have 
\begin{align}
    \E\left\{ \lambda_{N}^1(s)\right\} \leq 2 \widebar{\mathcal{R}}_{n}\left\{ \mathcal{G}_{N}^1(s) \right\}
    ~~\text{and}~~
    \E\left\{ \lambda_{N}^2(s)\right\} \leq 2 \widebar{\mathcal{R}}_{m}\left\{ \mathcal{G}_{N}^2(s) \right\}.
\end{align}
Since both $\phi_{*}\circ \phi'$ and $ \phi'$ are $L$-Lipschitz continuous, by the Ledoux-Talagrand contraction inequality due to \cite{ledoux1991}, it holds that $\widebar{\mathcal{R}}_{n}\left\{ \mathcal{G}_{N}^1(s) \right\} \leq 2 L\widebar{\mathcal{R}}_{n}(s, \mathcal{F}_{N}^*)$ and  $\widebar{\mathcal{R}}_{m}\left\{ \mathcal{G}_{N}^2(s) \right\} \leq 2 L\widebar{\mathcal{R}}_{m}(s, \mathcal{F}_{N}^*)$.  Therefore, 
\begin{align}
    \E\left\{ \lambda_{N}^1(s)\right\} \leq 4 L \widebar{\mathcal{R}}_{n}(s, \mathcal{F}_{N}^*) 
    ~~\text{and}~~
    \E\left\{ \lambda_{N}^2(s)\right\} \leq  4L \widebar{\mathcal{R}}_{m}(s, \mathcal{F}_{N}^*). \nn % \leq 4L (\delta_{n} + \delta_{m}),
\end{align}
{Since $\mathcal{F}_{N}^*$ is star-shaped around $r_{N}$ (if $r \in \mathcal{F}_{N}^*$, then for any $\alpha \in (0,1)$,  $\alpha r \in \mathcal{F}_{N}^*$),}
%\fn{{add an assumption?}}
the function $\widebar{\mathcal{R}}_{n}(s, \mathcal{F}_{N}^*) / s$ is non-increasing with resepct to $s$ according to Lemma 13.6 of \cite{wainwright2019}. As $s > \delta_{n}$ and $\delta_{n}^2 > \widebar{\mathcal{R}}_{n}\left\{\delta_{n}, \mathcal{F}_{N}^*\right\}$, it holds that $\widebar{\mathcal{R}}_{n}(s, \mathcal{F}_{N}^*) \leq s \delta_{n}$. Similarly, we also have $\widebar{\mathcal{R}}_{m}(s, \mathcal{F}_{N}^*) \leq s \delta_{m}$ for $s \geq \delta_{m}$ , which delivers the upper bounds % of $\E\left\{ \lambda_{N}(s)\right\}$:  
\begin{align}
    \E\left\{ \lambda_{N}^1(s)\right\} \leq   4 L s \delta_{n}
    ~~\text{and}~~
    \E\left\{ \lambda_{N}^2(s)\right\} \leq  4 L s \delta_{m} ~~(\forall s \geq \delta_{n} \vee \delta_{m}). 
    \label{eq: mean ep lr}
\end{align}

We next bound the deviation between  $\lambda_{N}^j(s)$  and $\E\left\{ \lambda_{N}^j(s)\right\}$ for $j = 1$ and $2$.   %To this end we write $\widehat{d}_{\phi}(r, r_{N}) = \P_{N}\left\{\ell_{\phi}(r) - \ell_{\phi}(r_0) \right\} $ and $d_{\phi}(r, r_{N}) = \E_{F}\left\{\ell_{\phi}(r) - \ell_{\phi}(r_0) \right\}$, where $\ell_{\phi}(r) = \frac{1-\delta}{1-p} \phi_{*}\left\{ \phi'(r(\bx))\right\} - \frac{\delta}{p} \phi'(r(\bx))$.  
Note that for any $r \in \mathcal{R}_{N}$, we have $\norm{\ell_{j}(r) - \ell_{j}(r_N)}_{\infty} \leq L \norm{r - r_{N}}_{\infty} \leq 2BL$, by the Lipschitz condition of $\phi_{*}\circ \phi'$ and $\phi'$ and the boundness of  $r \in \mathcal{R}_{N}$. In addition,      
the variance of $\ell_{j}(r) - \ell_{j}(r_N)$ can be upper bounded by  
\begin{align}
    \var(\ell_{j}(r) - \ell_{j}(r_N)) \leq & \E\left\{ (\ell_{j}(r) - \ell_{j}(r_N))^2 \right\} \nn \\ 
     \leq & L^2\left(\norm{r- r_{N}}_{L_{2}(P)}^2 + \norm{r- r_{N}}_{L_{2}(Q)}^2 \right) \nn \\ 
     \leq &  2(BL)^2 \norm{r- r_{N}}_{L_{2}(P)}^2 \leq 2 (BLs)^2,
     \label{eq: var ep lr}
\end{align}
where the second inequality is implied by the Lipschitz condition, the third inequality is due to $\norm{f}_{L_{2}(Q)}^2 = \norm{f\cdot r_{0}}_{L_{2}(P)}^2 \leq B^2 \norm{f}_{L_{2}(P)}^2$ for any $f: \mathcal{X}\to \mathbb{R}$, and the last inequality is because of %the curvature condition $\norm{r- r_{0}}_{L_{2}(P)}^2 \leq c_{1} d_{\phi}(r, r_{N}) \leq c_{1}s^2$. 
the localization condition ${\norm{r- r_{N}}_{L_{2}(P)} \lesssim \dphi(r, r_{N}) \leq s}$.  
Consequently, for any $u > 0$ it holds that %we find that there is a universal constant $c_{t}$ such that 
\begin{align}
    \P\left\{\lambda_{N}^j(s) \geq \E\{ \lambda_{N}^j(s)\} + u \right\} \leq &  2 \exp\left(\frac{- (n \wedge m) u^2}{8 e \var(\ell_{\phi}(r) - \ell_{\phi}(r_0)) + 8 BL u}\right) \nn \\ 
    \leq & 2 \exp\left(- \frac{C_{t} (n \wedge m) u^2}{(BLs)^2 + BLu}  \right),
    \nn
\end{align}     
for some universal constant $C_{t} > 0$, %by plugging in  \eqref{eq: mean ep lr} and \eqref{eq: var ep lr}. Consequently, we obtain the control on the upper tail of $\lambda_{N}(s)$: 
by applying Talagrand's concerntration equality (\citealp{talagrand1994}) and  \eqref{eq: var ep lr}. Therefore, we have   
\begin{align}
   \left(
    \P\left\{\lambda_{N}^1(s) \geq 4 L s \delta_{n}  + u \right\}
    \vee \P\left\{\lambda_{N}^2(s) \geq 4 L s \delta_{m}  + u \right\}
   \right)     \leq  2 \exp\left(- \frac{C_{t} (n \wedge m) u^2}{(BLs)^2 + BLu}  \right), \nn 
\end{align} 
for any $s \geq (\delta_{n} \vee \delta_{m})$ and $u > 0$.  
Since 
\[
\lambda_{N}(s) \leq \lambda_{N}^1(s) + \lambda_{N}^2(s)%~~\forall s > 0,
\]
for any $s \geq 0$,  
we have 
\begin{align}
    \P\left\{\lambda_{N}(s) \geq 4 L s( \delta_{n} + \delta_{m})  + u \right\} \leq 4  \exp\left(- \frac{C_{t} (n \wedge m) u^2}{(2BLs)^2 + 2BLu}  \right),
\end{align} 
for any $s \geq (\delta_{n} \vee \delta_{m})$ and $u > 0$.  
Denoting $\delta_{N}:=\delta_{n} + \delta_{m}$ 
and setting $s = \delta_{N}, u =B L  \delta_{N}^2$, then we have 
\begin{align}
    \P\left\{\lambda_{N}(\delta_{N}) \geq C_{1}   \delta_{N}^2 \right\} \leq  4 \exp\left(- C_{2} (n \wedge m) \delta_{N}^2  \right), 
    \label{eq: lambda-N tail-1}
\end{align}
where $C_{1} = (4 + B)L$ and $C_2 = C_t /6$. 
In addition, setting $u = BL s \delta_N$ yields 
\begin{align}
    \P\left\{\lambda_{N}(s) \geq C_{1}  s \delta_{N} \right\} \leq  2 \exp\left(- \frac{C_{t} n s^2 \delta_N^2}{s^2 + s \delta_N}  \right) \leq  4 \exp\left(- C_{2} (n \wedge m) \delta_{N}^2  \right),
    \label{eq: lambda-N tail-2}
\end{align}
for any $s \geq \delta_N$. 

{Let 
\begin{align}
    \mathcal{A}_{1} = \left\{ \exists~ r \in \mathcal{R}_{N}: 
    {\norm{r- r_{N}}_{L_{2}(P)} \leq \delta_{N}} ~~\text{and}~~
    \abs{\widehat{d}_{\phi}(r, r_{N}) - d_{\phi}(r, r_{N}) } \geq C_1 \delta_N^2
    \right\}. 
    \label{eq: A_1}
\end{align}
Combining  \eqref{eq: lambda_N(s)} with \eqref{eq: lambda-N tail-1} yields that 
\begin{align}
    \P(\mathcal{A}_{1} )\leq  4 \exp\left(- C_{2} (n \wedge m) \delta_{N}^2  \right).
    \label{eq: A_1 bound}
\end{align}
The above tail bound \eqref{eq: lambda-N tail-2} controls the largest deviation $\abs{\widehat{d}_{\phi}(r, r_{N}) - d_{\phi}(r, r_{N}) }$ for $r$  within the local ball $d_{\phi}(r, r_{N}) \leq \delta_N$.}
It remains to estimate an tail bound of the deviation $\abs{\widehat{d}_{\phi}(r, r_{N}) - d_{\phi}(r, r_{N}) }$ outside this local region. We define  the following event 
\[
\mathcal{A}_{2} = \left\{ \exists~ r \in \mathcal{R}_{N}:{\norm{r- r_{N}}_{L_{2}(P)} > \delta_{N}} ~~\text{and}~~  \abs{\widehat{d}_{\phi}(r, r_{N}) - d_{\phi}(r, r_{N}) } \geq 2 C_{1} \delta_{N} \norm{r- r_{N}}_{L_{2}(P)} \right\} 
\] 
However, bounding $\P(\mathcal{A}_{2})$ is more delicate, since the function $r$ that satisfies the requirement in $\mathcal{A}_{2}$  is random. %, we cannot just set $s =\norm{r- r_{N}}_{L_{2}(P)}$ in  \eqref{eq: lambda-N tail-2}, since it only applies to a deterministic $s$. 
In the following step, we will use a ``peeling'' argument to address the probelm.  

\bigskip
\ni {\bf Step 3: Bound the event $\mathcal{A}_{2}$ with the peeling argument.}
For $m \in \mathbb{N}_{+}$, we define the events 
\[
\mathcal{S}_{m} := \left\{ r \in \mathcal{R}_{N}: 2^{m-1} \delta_{N} < \norm{r- r_{N}}_{L_{2}(P)}  \leq 2^{m} \delta_{N}  \right\}.  
\]  
By the boundness of $r \in \mathcal{R}_{N}$, we have $\norm{r- r_{N}}_{L_{2}(P)} \leq 2 B$. Hence, any $r \in \mathcal{R}_{N} \cap \left\{  \norm{r- r_{N}}_{L_{2}(P)} > \delta_{N} \right\}$ must locate in some $\mathcal{S}_{m}$ for $m \in \iset{M}$, where $M \leq 2 \log(B / \delta_{N}) + 1$.      
Since $\mathcal{A}_{2}$ is a subset of $\cup_{m=1}^M S_{m}$, by the union bound we have $\P(\mathcal{A}_{2}) \leq \sum_{m=1}^M \P\left(\mathcal{A}_{2}\cap S_{m}\right)$. 

Note that if $r_{m} \in \mathcal{A}_{2}\cap S_{m}$, then we can take $s_{m} = 2^{m}\delta_{N}$, and $r_{m}$ satisfies  
$$
\norm{r_{m}- r_{N}}_{L_{2}(P)} \leq s_{m}~~\text{and}~~ \abs{\widehat{d}_{\phi}(r_{m}, r_{0}) - d_{\phi}(r_{m}, r_{0}) } \geq 2 C_{1}  \delta_{N} \norm{r- r_{N}}_{L_{2}(P)}  > C_{1} \delta_{N} s_{m},
$$  
where the last inequality is due to $2 \norm{r- r_{N}}_{L_{2}(P)} > 2^{m+1} \delta_{N} > s_{m} = 2^{m} \delta_{N}$. As a result, 
$
\mathcal{A}_{2} \cap \mathcal{S}_{m} \subset \left\{ \lambda_{N}(s_{m}) \geq C_{1} s_{m} \delta_{N}\right\}.  
$
Then according to \eqref{eq: lambda-N tail-2}, we obtain 
\begin{align}
  \P(\mathcal{A}_{2} ) & \leq \sum_{m=1}^M  \P(\mathcal{A} \cap \mathcal{S}_{m} ) \leq 2 \sum_{m=1}^M  \exp\left(- C_{2} (n \wedge m) \delta_{N}^2  \right) \nn \\  & = 4 \exp(- C_{2} (n \wedge m) \delta_{N}^2  + \log M) \leq 4 \exp\left(- \frac{C_{2} (n \wedge m) \delta_{N}^2 }{2}\right),
  \label{eq: A_2 bound}
\end{align}
where the last inequality holds provided that 
\begin{align}
    \frac{C_{2} (n \wedge m) \delta_{N}^2 }{2} \geq \log\left(2\log(B / \delta_{N}) + 1\right).
\end{align}

\iffalse
In the case that $d_{\phi}(r_{N}, r_{0}) < \delta_{N}^2$, then \eqref{A_1} and \eqref{A_1 bound} imply that 
\[
\P\left\{ \abs{\widehat{d}_{\phi}(r_{N}, r_{0}) - d_{\phi}(r_{N}, r_{0}) } \geq C_{1}\delta_{N}^2 \right\} \leq 4 \exp\left(- \frac{C_{2} (n \wedge m) \delta_{N}^2 }{2}\right). 
\] 
Otherwise, in the case that $d_{\phi}(r_{N}, r_{0}) \geq \delta_{N}^2$, then \eqref{eq: A_2 bound} implies that 
\[
    \P\left\{ \abs{\widehat{d}_{\phi}(r_{N}, r_{0}) - d_{\phi}(r_{N}, r_{0}) } \geq 2 C_{1}  \delta_{N} \sqrt{d_{\phi}(r_{N}, r_{0})}  \right\} \leq 4 \exp\left(- \frac{C_{2} (n \wedge m) \delta_{N}^2 }{2}\right). 
\] 
Since $2 C_{1}  \delta_{N} \sqrt{d_{\phi}(r, r_{N})}  \leq C_{1}^2 \delta_{N}^2  + d_{\phi}(r, r_{N})$, combining the two cases we obtain
\[
    \P\left\{ \abs{\widehat{d}_{\phi}(r_{N}, r_{0}) - d_{\phi}(r_{N}, r_{0}) } \geq C_{4} \left(\delta_{N}^2  + d_{\phi}(r_{N}, r_{0})\right)  \right\} \leq 4 \exp\left(- \frac{C_{2} (n \wedge m) \delta_{N}^2 }{2}\right),
\]  
where $C_{4} = (C_{1} \vee C_{1}^2)$.  
\fi

The complement of $\mathcal{A}_{2}$ is composed by $\mathcal{A}^c_{2} = \mathcal{B}_{1} \cup \mathcal{B}_{2}$, where 
\[
\mathcal{B}_{1} = \left\{r \in \mathcal{R}_{N}: ~  \norm{r- r_{N}}_{L_{2}(P)} \leq \delta_{N}\right\}~~\text{and}~~
\mathcal{B}_{2} = \left\{r \in \mathcal{R}_{N}: ~  \abs{\widehat{d}_{\phi}(r, r_{N}) - d_{\phi}(r, r_{N}) } < 2 C_{1} \delta_{N}  \norm{r- r_{N}}_{L_{2}(P)} \right\}.   
\]    
Therefore, \eqref{eq: A_2 bound} implies that 
\begin{align}
    \P(\mathcal{B}_{1} \cup \mathcal{B}_{2} )\geq 1 - 4 \exp\left(- \frac{C_{2} (n \wedge m) \delta_{N}^2 }{2}\right). \nn 
\end{align}
If $\widehat{r} \in \mathcal{B}_{1}$, then we have $ d(\widehat{r}, r_{N}) \leq c_{2}^{-2} \delta_{N}$ since  $d(\widehat{r}, r_{N}) \leq c_{2} \norm{\widehat{r}- r_{N}}_{L_{2}(P)}^2$.  
Moreover, if $\widehat{r} \in \mathcal{B}_{2}$, since $ c_{1}\norm{\widehat{r} -r_{N}}_{L_{2}(P)}^2 \leq  d_{\phi}(\widehat{r}, r_{N}) $, and $\widehat{d}(\widehat{r}, r_{N}) \leq 0$ by the definition of $\widehat{r}$,  we have
$
d_{\phi}(\widehat{r}, r_{N})  < 4 c_{1}^{-2}C_{1}^2 \delta_{N}^2.
$ Therefore, we conclude that 
\begin{align}
    \P\left\{d_{\phi}(\widehat{r}, r_{N}) < (c_{2}^{-2} \vee  4 c_{1}^{-2}C_{1}^2) \delta_{N}^2 \right\} \geq 
    1 - 4 \exp\left(- \frac{C_{2} (n \wedge m) \delta_{N}^2 }{2}\right). 
    \label{eq: d(r, rN) tail}
\end{align} 
Let $C_{3} = c_{2}^{-2} \vee  4 c_{1}^{-2}C_{1}^2$ and $C_{4} = C_{2} / 2$, combining  \eqref{eq: hat-r-decom} and \eqref{eq: d(r, rN) tail}, we obtain 
\begin{align}
    \P\left\{ c_{1}\norm{\widehat{r} -r_{0}}_{L_{2}(P)}^2 \leq C_{3} \delta_{N}^2 +c_{2} \varepsilon_{N}^2   \right\}
    \geq 
    1 - 4 \exp\left(- \frac{C_{2} (n \wedge m) \delta_{N}^2 }{2}\right). 
    \label{eq: hat-r-bound-1}
\end{align}
Therefore, the estimation error $\norm{\widehat{r} -r_{0}}_{L_{2}(P)}$ relies on the critical radius $\delta_{N}$ and the approximation error $\varepsilon_{N}$. In the next step, we provide an upper bound of the critical radius $\delta_{N}$. 

\ni {\bf Step 4: Estimation of the critical radius $\delta_{N}$.}
%Recall that $\delta_{N} = \delta_{n} + \delta_{m}$, where $\delta_{n}, \delta_{m}$ are the smallest solutions of
%\begin{align}
%    \delta_{n}^2 \geq  \widebar{\mathcal{R}}_{n}(\delta_{n}, \mathcal{F}^*_{N} ), ~~~  \delta_{m}^2 \geq  \widebar{\mathcal{R}}_{m}(\delta_{m}, \mathcal{F}^*_{N} ),
%%    \label{eq: pop critic radius}
%\end{align} 
%respectively. However, the localized population Rademacher complexities $\widebar{\mathcal{R}}_{n}(\delta_{n}, \mathcal{F}^*_{N} )$ and $\widebar{\mathcal{R}}_{n}(\delta_{m}, \mathcal{F}^*_{N} )$ tend to be more difficult to estimate compared with the localized empirical Rademacher complexities $\widehat{\mathcal{R}}_{n}(\delta_{n}, \mathcal{F}^*_{N} )$ and $\widehat{\mathcal{R}}_{n}(\delta_{m}, \mathcal{F}^*_{N} )$. Therefore, 
In this step, we  first estimate the empirical critical radiuses $ \widehat{\delta}_{n}$ and $ \widehat{\delta}_{m}$   satisfying 
\begin{align}
    \widehat{\delta}_{n}^2 \geq  \widehat{\mathcal{R}}_{n}(\widehat{\delta}_{n}, \mathcal{F}^*_{N} ), ~~~  \widehat{\delta}_{m}^2 \geq  \widehat{\mathcal{R}}_{m}(\widehat{\delta}_{m}, \mathcal{F}^*_{N} ),
    \label{eq: emp critic radius}
\end{align} 
where $\widehat{\mathcal{R}}_{n}(\delta_{n}, \mathcal{F}^*_{N} )$ and $\widehat{\mathcal{R}}_{n}(\delta_{m}, \mathcal{F}^*_{N} )$ are localized empirical Rademacher complexities,
then use Proposition 14.25 of \cite{wainwright2019} to obtain that 
%\fn{\han{Need a lemma to extend this proposition to our loss functions}}
\begin{align}
    \P( C_{4} \delta_{n} \leq \widehat{\delta}_{n} \leq C_5 \delta_{n} ) \geq 1 - C_{6} \exp(-C_{7} n \delta_{n}^2)
    \label{eq: deviation of radius}
\end{align}
for some generic constants $C_{4}, \cdots, C_{7} > 0 $. 

By the Dudley's chaining, we have 
\begin{align}
    \widehat{\mathcal{R}}_{n}(s, \mathcal{F}^*_{N} )  % = \E_{\varepsilon} R_{n}\left\{f: f \in \mathcal{F}_{N}^*, ~ \norm{f}_{n} \leq \delta \right\} 
    \leq \inf_{0 < \alpha < s}\left\{ 4 \alpha + \frac{12}{\sqrt{n}} \int_{\alpha}^s \sqrt{\log\left(\mathcal{N}_{2}(\varepsilon, \mathcal{F}^*_{N}, \bX_{1}^n ) d \varepsilon \right)}  \right\},
    \label{eq: Dudley}
\end{align}
where $\bX_{1}^n = (\bX_{1},\cdots , \bX_{n})$. Since for any $\norm{f}_{n} \leq \max_{1 \leq i \leq n}\abs{f(\bX_{i})}$, we have $\mathcal{N}_{2}(\varepsilon, \mathcal{F}^*_{N}, \bX_{1}^n ) \leq \mathcal{N}_{\infty}(\varepsilon, \mathcal{F}^*_{N}, \bX_{1}^n )$.  
Since $\norm{f}_{\infty} \leq 2M$ for $f \in \mathcal{F}_{N}^*$,  
according to Theorem 12.2 of \cite{anthony1999neural}, we have 
\[
\log\left(\mathcal{N}_{\infty}(\varepsilon, \mathcal{F}^*_{N}, \bX_{1}^n ) \right) \leq \pdim(\mathcal{F}_{N}^*)\left(\frac{4 e M n }{\varepsilon \pdim(\mathcal{F}_{N}^*) }\right). 
\] 
When $ n > \pdim(\mathcal{F}_{N}^* )$,   let $\alpha =  s  \sqrt{\pdim(\mathcal{\mathcal{F}_{N}^*} ) / n}$ in \eqref{eq: Dudley}, we have 
\begin{align}
    \inf_{0 < \alpha < s}\left\{ 4 \alpha + \frac{12}{\sqrt{n}} \int_{\alpha}^s \sqrt{\log\left(\mathcal{N}_{2}(\varepsilon, \mathcal{F}^*_{N}, \bX_{1}^n ) d \varepsilon \right)}  \right\} \leq 16 s 
    \sqrt{ \frac{\pdim(\mathcal{F}_{N}^* )}{n} \left(\log \frac{4e M }{s} + \frac{3}{2}\log n\right)}. \nn 
\end{align}
Therefore, if $s \geq 1 / n$ and $n \geq (4eM)^2$, the localized empirical Rademacher complexity can be upper bounded by 
\begin{align}
    \widehat{\mathcal{R}}_{n}(s, \mathcal{F}^*_{N} ) \leq 32 s 
    \sqrt{ \frac{\pdim(\mathcal{F}_{N}^* )}{n} \log(n)}. \nn 
\end{align}  
With such result, we find that the $\widehat{\delta}_{n}$ satisfying $\widehat{\delta}_{n}^2 \geq \widehat{\mathcal{R}}_{n}(\widehat{\delta}_{n}, \mathcal{F}^*_{N} )$ can be taken as 
\begin{align}
    \widehat{\delta}_{n} = 32  \sqrt{ \frac{\pdim(\mathcal{F}_{N}^* )}{n} \log(n)} = 32  \sqrt{ \frac{\pdim(\mathcal{F}_{N} )}{n} \log(n)} . 
    \label{eq: empirical critical}
\end{align}
\iffalse
As $\mathcal{F}_{N}^* = \left\{ r - r_{N}: r \in \mathcal{R}_{N} \right\}$, the pseudo-dimension of $\mathcal{F}_{N}^*$ is the same of that of $\mathcal{R}_{N}$, which can be bounded by 
\[
\pdim(\mathcal{R}_{N} ) \leq C_{8} S_{N} L_{N} \log(S_{N}), 
\]     
where $S_{N}$ is the total number of parameters of the networks in $\mathcal{R}_{N}$. Therefore, the empirical critical radius $\widehat{\delta}_{n}$ can be bounded by 
\[
    \widehat{\delta}_{n} \leq C_{9} \sqrt{ S_{N} L_{N} \log(S_{N}) \frac{\log(n)}{n}} =: \zeta_{n} ,
\] 
where $C_{9} = 32 \sqrt{C_{8}}$. 
\fi
The empirical critical value $\hat{\delta}_m$ can be taken similarly. 
Using \eqref{eq: hat-r-bound-1}, \eqref{eq: deviation of radius}, and \eqref{eq: empirical critical}, we obtain that for any $u \geq 0$, 
\begin{align}
    \P\left\{ \norm{\widehat{r} -r_{0}}_{L_{2}(P)}^2 \leq C_8  \left(\xi_N+ \epsilon_N^2 + u\right)\right\} \geq 1 - C_9 \exp(-N \xi_N - Nu),
    \label{eq:C21}
\end{align}
for some universal constants $C_8$ and $C_9 > 0$,
where $\xi_N$ represents the stochastic error in the estimation and is defined as 
\[
\xi_N = \pdim(\mathcal{F}_{N} ) \left(\frac{\log(n)}{n} + \frac{\log(m)}{m} \right).
\]
Since $N\xi_N \asymp  \pdim(\mathcal{F}_{N} ) \log(N)$, we have $\exp(-N \xi_N) < C_9$ for  large enough $N$. Therefore, \eqref{eq:C21} implies that for large enough $N$ and any $t \geq 0$, it holds that 
\[
\P\left\{ \norm{\widehat{r} -r_{0}}_{L_{2}(P)}^2 \leq C_8  \left(\xi_N+ \epsilon_N^2 + \frac{1}{t}\right)\right\} \geq 1 -\exp(-t),
\]
which completes the proof.

\section{Proofs for Section \ref{sec: m3}}
\label{sec: proof for mi}
%\subsection{Proof of Theorem \ref{thm: conv rate of cde}}

For any given distribution $\tilde{P}_Y$ supported on $\mathbb{R}$ with a known density $\tilde{p}_0(y)$, we let $\tilde{P} = \tilde{P}_Y \times P_{\bX}$ be the distribution of $(\tilde{Y}, \bX)$ for $\bX \sim \P_{\bX}$ and $Y \sim \tilde{P}_Y$, which is independent of $\bX$, and let
\[
\tilde{r}_0(y, \bx) = \frac{p_0(y, \bx)}{p_0(\bx)\tilde{p}_0(y) },
\]
be the true density ratio function between $P$ and $\tilde{P}$. Then, under Conditions \ref{con: tilde-p} and \ref{con: app G},  applying Theorem \ref{thm: conv-r} leads to 
\begin{align}
    \norm{\hat{r} - \tilde{r}_0}_{L_2(\tilde{P})} = O_p\left(n^{-\frac{\beta_2}{2\beta_2 + d + 1}}\sqrt{\log (n)}\right),
\end{align}
for the estimator $\hat{r}$ defined in \eqref{eq: cde-r}. Since $\hat{p}(y, \bx) = \hat{r}(y, \bx)\tilde{p}_0(y)$ and $p_{Y|\bX}(y, \bx) = \tilde{r}_0(y, \bx)\tilde{p}_0(y)$, we have
\[
\hat{p}(y, \bx) = \hat{r}(y, \bx)\tilde{p}_0(y)
\]

\subsection{Proof of Theorem \ref{thm: conv rate of mi}}

For any $\btheta$, let  $\wh{\bbm}(\bX, \btheta) = \int \bg(y, \bX, \btheta) \hat{p}(y | \bX) dy$ be the conditional mean function with the estimarted conditional density function $\hat{p}(y | \bX)$, then 
\begin{align}
 \norm{\wh{\bbm}(\bX, \btheta) - \bbm_{0}(\bX, \btheta)}_{L_{2}(P_{\bX})} = \left( \E_{\bX}\left[ \int g(y, \bX, \btheta) \{\hat{p}(y | \bX) - {p}_{Y|\bX}(y | \bX)  \} dy \right]^2\right)^{\frac{1}{2}}. \nn 
\end{align}  
Since there exists a constant $m > 0$ such that $p_0(y |\bX) > m$, we have 
\begin{align}
    &~~~ \left\{ \int |\bg(y, \bX, \btheta)| |\hat{p}(y | \bX) - {p}_{Y|\bX}(y | \bX)  | dy \right\}^2 \nn \\ & \leq m^{-1}\left\{ \int |\bg(y, \bX, \btheta)| |\hat{p}(y | \bX) - {p}_{Y|\bX}(y | \bX) | \sqrt{p_{Y|\bX}(y | \bX)} dy \right\}^2 \nn \\ 
    & \leq m^{-1} \int g^2 (y, \bX, \btheta) |\hat{p}(y | \bX) - {p}_{Y|\bX}(y | \bX)  |^2 dy \int p_{Y|\bX}(y | \bX) dy  \nn \\
    & \leq m^{-1}\log^2(n) \int  |\hat{p}(y | \bX) - {p}_{Y|\bX}(y | \bX)  |^2 dy +  \nn \\ 
    &~~+  m^{-1} \int g^2(y, \bX, \btheta) I(|g^2(y, \bX, \btheta)| > \log n ) |\hat{p}(y | \bX) - {p}_{Y|\bX}(y | \bX)  |^2 dy \nn \\ 
   % & \leq  m^{-1}\log^2(n)  O_p(n^{- \frac{2s}{2s + d}}) + \nn \\ 
   % & ~~+ m^{-1} \int g^2(y, \bX, \btheta) I(|g^2(y, \bX, \btheta)| > \log n ) |\hat{p}(y | \bX) - {p}_{Y|\bX}(y | \bX)  |^2 dy \nn 
   & =: I_{1} + I_{2}, ~~\text{say}. 
\end{align}
Note that as $\hat{p}(y | \bX) $ and ${p}_{Y|\bX}(y | \bX) $ are uniformaly bounded by a constant $M > 0$, we have 
\begin{align}
    |\hat{p}(y | \bX) - {p}_{Y|\bX}(y | \bX)  |^2 \leq 4 M^2 + M p_0(y | \bX) \leq (4M^2 m^{-1} + M) p_0(y | \bX).  
\end{align}
Hence, $I_{2}$ can be bounded by 
\begin{align}
    I_{2} = & \int g^2(y, \bX, \btheta) I(|g^2(y, \bX, \btheta)| > \log n ) |\hat{p}(y | \bX) - {p}_{Y|\bX}(y | \bX)  |^2 dy \nn \\  
\lesssim & \int g^2(y, \bX, \btheta) I(|g^2(y, \bX, \btheta)| > \log n )  p_0(y | \bX)dy \nn \\ 
    \lesssim & \left\{ \left(\int g^4(y , \bX) p_0 (y | \bX) dy\right) \left(\int  I(|g^2(y, \bX, \btheta)| > \log n )p_0 (y | \bX) dy \right)  \right\}^{1/2} \nn \\ 
    \lesssim & n^{-1}, 
\end{align}
almost surely,
which implies $ \E_{\bX}(I_{2})  \lesssim  n^{-1}$, where the expectation is taken with respect to $\bX$ but not with respect to  $\hat{p}$.
%Therefore, we obtain that 
%\[
%  \left[ \int |\bg(y, \bX, \btheta)| |\hat{p}(y | \bX) - {p}_{Y|\bX}(y | \bX)  | dy \right]^2 \leq C_1(M, m, \sigma_g) \log^2(n)  O_p(n^{- \frac{2s}{2s + d}}). 
%\]
%Because $\mathcal{X}_P$ is compact and $f_0(\bx)$ is bounded, the DCT leads to 
%\[
% \E_{\bX}\left[ \int \bg(y, \bX, \btheta) \{\hat{p}(y | \bX) - {p}_{Y|\bX}(y | \bX)  \} dy \right]^2 = O_p(\log^2(n) n^{- \frac{2s}{2s + d}}). 
%\]
For the $I_{1}$ term, we have 
\begin{align}
    \E_{\bX}(I_{1}) & = m^{-1}\log^2(n)  \int |\hat{p}(y | \bx) - {p}_{Y|\bx}(y | \bX)  |^2 p_{0}(\bx) dy d\bx \nn \\ 
& \lesssim \log^2(n)  \int |\hat{p}(y | \bx) - {p}_{Y|\bx}(y | \bX)  |^2 p_{0}(\bx) \tilde{p}_{Y}(y) dy d\bx \nn \\ 
& = \log^2(n) \E_{(\tilde{Y},\bX)}\left\{\hat{p}(\tilde{Y}|\bX) -  {p}_{Y|\bx}(\tilde{Y} | \bX) \right\}^2 \nn \\ 
& = O_{p}\left(\log^3(n) n^{-\frac{2\beta_{2}}{2\beta_{2} + d+1}} \right),  
\end{align} 
where the inequality is by the uniform boundness of $ \tilde{p}_{Y}$, and the last equality is due to Theorem \ref{thm: conv rate of cde}. Hence, $\norm{\wh{\bbm}(\bX, \btheta) - \bbm_{0}(\bX, \btheta)}_{L_{2}(P_{\bX})} = \E_{\bX}(I_{1}) + \E_{\bX}(I_{2}) =  O_{p}\left(\log^3(n) n^{-\frac{2\beta_{2}}{2\beta_{2} + d+1}} \right)$, which together with the use of Chebyshrev's inequality complete the proof of Theorem \ref{thm: conv rate of mi}.

\section{Proofs for Section \ref{sec: theory-el}}

Given the estimated $\wh{\bfeta}$, for any $\btheta$, we let $\bPsi_i(\btheta, \wh{\bfeta}) = \bPsi(\bW_i, \btheta, \bfeta)$, $\wh{\bPsi}(\btheta, \wh{\bfeta}) = N^{-1}  \sum_{i = 1}^N \bPsi_i(\btheta,  \wh{\bfeta})$, and $\wh{\Omega}(\btheta, \bfeta) =  N^{-1} \sumiN \bPsi_i(\btheta,  \wh{\bfeta}) \bPsi_i(\btheta,  \wh{\bfeta})\t$. With the EL estimator $\wh{\btheta}$, we write $\bPsi_i(\wh{\bfeta}) = \bPsi_i(\wh{\btheta}, \wh{\bfeta})$, $\wh{\bPsi}(\wh{\btheta}, \wh{\bfeta}) = \wh{\bPsi}(\wh{\btheta}, \wh{\bfeta})$, and $\wh{\Omega}(\bfeta) = \wh{\Omega}(\wh{\btheta}, \bfeta)$. %For any $\xi \in (1/\alpha, 1/2)$, let $\Lambda_N = \{\lambda \in \mathbb{R}^r: \norm{\lambda} \leq N^{-\xi}\}$. 

\begin{lem} \label{lem: E.1}
     Under Conditions \ref{con: dist} and \ref{con: moment function}, if the estimation errors satisfy  
    \begin{equation} \mathcal{E}_N(\widehat{r})+\mathcal{E}_N(\widehat{\bbm}_{\btheta})= o_{p}(1)~~\text{and}~~\mathcal{E}_N(\widehat{r})\mathcal{E}_N(\widehat{\bbm}_{\btheta}) = o_{p}(N^{-\frac{1}{2}}),
        \label{eq: con of errors}
    \end{equation}
    then we have
\iffalse
\begin{align}
    \frac{1}{\sqrt{N}}\sum_{k=1}^K\sum_{i \in \mathcal{I}_{k}}  \bPsi(\bW_i, \btheta_{0}, \widehat{\bfeta}) =  \frac{1}{\sqrt{N}}\sum_{i=1}^N \bPsi(\bW_i, \btheta,\bfeta) + o_{p}(1). 
\end{align}
\fi 
\begin{align}
    \frac{1}{\sqrt{N}}\sum_{i=1}^N  \bPsi(\bW_i, \btheta, \wh{\bfeta}) =  \frac{1}{\sqrt{N}}\sum_{i=1}^N \bPsi(\bW_i, \btheta,\bfeta_{0}) + o_{p}(1). 
    \label{eq: E12}
\end{align}
\end{lem}
\begin{proof}
\iffalse
For every $k = 1,\dots, K$  and $i \in \mathcal{I}_{k}$, let $N_{k} = \sum_{i = 1}^N {I}(i \in \mathcal{I}_{k})$ be the sample size in the group $\mathcal{I}_{k}$ and  define $\bR_{ki} = \bPsi(\bW_i, \btheta_{0}, \widehat{\bfeta})  - \bPsi(\bW_i, \btheta_{0},\bfeta_{0}) = (R_{ki1},\dots, R_{kir})\t$, so that the result in Theorem 1 that we aim to show can be written as 
$
\frac{1}{\sqrt{N}} \sum_{k=1}^K\sum_{i\in \mathcal{I}_{k}} R_{kij} = o_{p}(1). 
$ 

Let $\mathcal{W}_{k}^c$ be the observations not in $I_{k}$, so that $\widehat{\bfeta}$ depend only on $\mathcal{W}_{k}^c$.  
Then 
\begin{align}
    \left|\frac{1}{\sqrt{N}}\sum_{i \in \mathcal{I}_{k}} \E(R_{kij}|\mathcal{W}_{k}^c) \right|
    &= \frac{N_{l}}{\sqrt{N}}\left| \E \{  \Psi_{j}(\bW_i, \btheta_{0}, \widehat{\bfeta}) | \mathcal{W}_{k}^c  \} \right| \nn \\ 
    & \leq \sqrt{N}\left| \E \{  \Psi_{j}(\bW_i, \btheta_{0}, \widehat{\bfeta}) | \mathcal{W}_{k}^c  \} \right|  \nn \\ 
    & \leq \sqrt{N}\mathcal{E}(\widehat{r}_{{-k}})\mathcal{E}(\widehat{m}_{-k,j})  = o_{p}(1),
    \label{eq: s9}
\end{align}
where the second inequality is by \eqref{eq: s8}, taking $\widehat{\bfeta}$ as a constant as the expectation is condtional on $\mathcal{W}_{k}^c$. We now show that the second conditional moment $\E(\widehat{R}_{kij}^2 | \mathcal{W}_{k}^c) = o_{p}(1)$.
\fi 

Note that for each $i = 1, \cdots, N$,  
\begin{align}
  &  \bPsi(\bW_{i}, \btheta, \widehat{\bfeta})  -   \bPsi(\bW_{i}, \btheta, \bfeta_{0}) = R_{1,i}(\wh{\bfeta}) + R_{2,i}(\wh{\bfeta}) + R_{3,i}(\wh{\bfeta}),   
\nn 
\end{align}
where 
\begin{align}
     R_{1,i}(\wh{\bfeta}) = & \left\{ \frac{\delta_i}{p}-\frac{1-\delta_i}{1-p}{r}_0(\bX_{i}) \right\} \{ \widehat{\bbm}(\bX_{i}, \btheta)\} -   {\bbm}(\bX_{i}, \btheta)\},  \nn \\ 
       R_{2,i}(\wh{\bfeta}) = &\frac{1-\delta_i}{1-p}\{\widehat{r}(\bX_{i}) - r_{0}(\bX_{i}) \} \{ \widehat{\bbm}(\bX_{i}, \btheta)\} -   {\bbm}(\bX_{i}, \btheta)\},  \nn \\ 
     R_{3,i}(\wh{\bfeta}) =&\frac{1-\delta_i}{1-p}\{\widehat{r}(\bX_{i}) - r_{0}(\bX_{i}) \} \{ \bg(\bZ_{i}, \btheta)  - {\bbm}_{0}(\bX_{i}, \btheta)\}. \nn 
\end{align}

Let $R_{j}(\wh{\bfeta}) = N^{-\frac{1}{2}} \sumiN R_{j,i}(\wh{\bfeta})$ for $j = 1, 2, 3$. Then \eqref{eq: E12} can be shown if $R_{j}(\wh{\bfeta}) = o_p(1)$  for $j = 1, 2, 3$. For the first term, 
\begin{align}
\E\{R_{1}^2(\wh{\bfeta}) | \{ \bX_i \}_{i=1}^N \}&  = \E_N \left[  \left\{ \frac{\delta_i}{p}-\frac{1-\delta_i}{1-p}{r}_0(\bX_{i}) \right\}^2  \{ \widehat{\bbm}(\bX_{i}, \btheta)\} -   {\bbm}(\bX_{i}, \btheta)\}^2 \right] \nn \\ 
& \lesssim \E_N \left[ \{ \widehat{\bbm}(\bX_{i}, \btheta)\} -   {\bbm}(\bX_{i}, \btheta)\}^2 \right] = \cE_N(\wh{\bbm}_{\btheta}) = o_p(1),
\end{align}
where the first equality is due to 
\begin{align}
    \E_N\{ R_{1,i}(\wh{\bfeta})R_{2,i}(\wh{\bfeta}) | \{ \bX_i \}_{i=1}^N  \}  = 0, \nn  
\end{align}
for each $ i \neq i'$,
by the independence of $(\bX_i, \delta_i)$  and $(\bX_i', \delta_i')$, and $\E_N \left\{ \frac{\delta_i}{p}-\frac{1-\delta_i}{1-p}{r}_0(\bX_{i})  | \bX_i\right\}  = 0$ for each  $1 \leq i  \leq N$. Therefore, $R_{1}(\wh{\bfeta}) = o_p(1)$. For the second term, we have 
\begin{align}
R_{2}(\wh{\bfeta}) & = \sqrt{N} \E_N \left\{\frac{1-\delta_i}{1-p}\abs{\widehat{r}(\bX_{i}) - r_{0}(\bX_{i}) } \abs{ \widehat{\bbm}(\bX_{i}, \btheta) -   {\bbm}(\bX_{i}, \btheta)} \right\} \nn \\ 
& \lesssim \sqrt{N} \cE_N(\wh{r}) \cE_N(\wh{\bbm}_{\btheta_0}) = o_p(1), \nn 
\end{align}
by the Cauchy-Schwarz inequality and \eqref{eq: con of errors}. Finally, for the third term, 
\begin{align}
\E\{R_{3}^2(\wh{\bfeta}) | \{\delta_i ,\bX_i \}_{i=1}^N \}&  = \E_N\left[ \frac{1-\delta_i}{(1-p)^2}\{\widehat{r}(\bX_{i}) - r_{0}(\bX_{i}) \}^2 \{ \bg(\bZ_{i}, \btheta_{0})  - {\bbm}_{0}(\bX_{i}, \btheta)\}^2 | \{\delta_i ,\bX_i \}_{i=1}^N \right] \nn \\ 
& \lesssim \E_n \left[\{\widehat{r}(\bX_{i}) - r_{0}(\bX_{i}) \}^2 \var(\bg(\bZ_i, \btheta)|\bX_i) \}_{i=1}^N \right] \nn \\
& \lesssim \cE_n(\wh{r}) = o_p(1). \nn 
\end{align}
Therefore, we have $R_{3}(\wh{\bfeta}) = o_p(1)$. Since 
\[ \frac{1}{\sqrt{N}}\sum_{i=1}^N  \bPsi(\bW_i, \btheta, \wh{\bfeta}) -  \frac{1}{\sqrt{N}}\sum_{i=1}^N \bPsi(\bW_i, \btheta,\bfeta) = R_{1}(\wh{\bfeta})+ R_{2}(\wh{\bfeta}) + R_{3}(\wh{\bfeta}),  \] the proof of Lemma \ref{lem: E.1} is finished.
\end{proof}

\begin{lem}
    Under Conditions \ref{con: dist} and \ref{con: moment function}, if the estimation errors satisfy  
    \begin{equation}
       \mathcal{E}_N(\widehat{r})+\mathcal{E}_N(\widehat{\bbm})= o_{p}(1)
        ~~\text{and}~~
        \mathcal{E}_N(\widehat{r})\mathcal{E}_N(\widehat{\bbm}) = o_{p}(N^{-\frac{1}{2}}).
        \label{eq: con of eta for AN}
\end{equation}
\end{lem}

\begin{proof}
The EL estimator $\wh{\btheta}$ can be written as the solution to the saddle point problem (\citealp{newey-smith-04}): 
\begin{align}
\wh{\btheta} = \argmin_{\btheta \in \Theta} \sup_{\lambda \in \wh{\Lambda}_N(\btheta)}   \aveiN \rho(\lambda\t \bPsi_i(\btheta, \wh{\bfeta})),
\label{eq: E.1}
\end{align}
where $\rho(v) = \log(1+v)$ and $\wh{\Lambda}_N(\btheta) = \{\lambda: \lambda\t \bPsi_i(\btheta, \wh{\bfeta}) \in (-1, \infty)\}$. For any $\xi \in (1/\alpha, 1/2)$ where $\alpha$ is defined in Condition \ref{con: dist} (ii), let $\tilde{\lambda} =  N^{-\xi}\wh{\bPsi}(\wh{\btheta}, \wh{\bfeta}) / \norm{\wh{\bPsi}(\wh{\btheta}, \wh{\bfeta}) }$.  By Lemma A1 of \cite{newey-smith-04}, $\max_{i\leq N} |\tilde{\lambda}\t \wh{\bPsi}_i(\hetak)| = o_p(1)$, and  $\tilde{\lambda} \in \Lambda_N(\wh{\btheta})$ with probability approaching $1$. Thus, for any $\dot{\lambda} \in (\tilde{\lambda},0)$. Let $\rho_{k}$ be the $k$-th derivative function of $\rho$. Then since $\rho_2(0) = -1$, with probability approaching $1$ we have $\rho_2(\dot{\lambda}\t \wh{\bPsi}_i(\hetak)) \geq -C (i=1, \cdots, N)$ for some positive constant $C_1$.  In addition, by the Cauchy-Schwarz inequality, Condition \ref{con: moment function} (ii), and the uniform weak law of large numbers it can easily be derived that $ N^{-1} \sumiN \bPsi_i(\btheta, \wh{\bfeta}))^{\otimes 2} \leq C_2 \bI_{r}$ for some positive constant $C_2$ with probability approaching $1$, meaning that the largest eigenvalue of $N^{-1}\sumiN \bPsi_i(\btheta, \wh{\bfeta})$ is bounded from above with probability approaching $1$. Taking the Taylor expansion for $\rho(\tilde{\lambda}\t \bPsi_i(\wh{\btheta}, \wh{\bfeta}))$ at $0$ gives 
\begin{align}
\aveiN \rho(\tilde{\lambda}\t \bPsi_i(\wh{\btheta}, \wh{\bfeta}))& = \tilde{\lambda}\wh{\bPsi}(\wh{\btheta}, \wh{\bfeta}) + \frac{1}{2} \tilde{\lambda}\t\left\{ \aveiN  \rho_2(\dot{\lambda}\t \wh{\bPsi}_i(\wh{\btheta}, \wh{\bfeta}))\bPsi_i(\wh{\btheta}, \wh{\bfeta}))^{\otimes 2}   \right\}\tilde{\lambda} \nn \\ 
& \geq N^{-\xi}\norm{\wh{\bPsi}(\wh{\btheta}, \wh{\bfeta})} - \frac{C_1C_2}{2} \norm{\tilde{\lambda}}^2 \geq N^{-\xi}\norm{\wh{\bPsi}(\wh{\btheta}, \wh{\bfeta})} - C_3 N^{-2\xi}, 
\label{eq: E.2}
\end{align}
with probability approaching $1$, where $C_3 = C_1 C_2 / 2$. 

By the similar arguments as Lemma A2 of \cite{newey-smith-04}, it can be shown that if for any $\bar{\btheta} \in \Theta$ such that $\bar{\btheta} = \btheta_0 + o_p(1)$ and $\wh{\bPsi}(\bar{\btheta}, \wh{\bfeta}) = O_p(N^{-\frac{1}{2}})$, then $$\bar{\lambda} = \argmax_{\lambda \in \wh{\Lambda}_N(\bar{\btheta})}  N^{-1} \aveiN  \rho(\lambda\t \bPsi_i(\bar{\btheta}, \wh{\bfeta}))$$ exists with probability approaching $1$,  also it holds that
\begin{align}
   \sup_{\lambda \in \wh{\Lambda}_N({\btheta}_0)} \aveiN \rho(\lambda\t \bPsi_i(\bar{\btheta}, \wh{\bfeta})) = O_p(N^{-1}), ~~\text{and}~~\bar{\lambda} = O_p(N^{-\frac{1}{2}}). 
   \label{eq: claim: EL}
\end{align}
Setting $\bar{\btheta} = \btheta_0$. 
%note that Theorem \ref{thm1} (iii) gives $\E\{ \wh{\bPsi}(\btheta_0, \wh{\bfeta})\} = o_p(1)$, which together with the CLT implies $\wh{\bPsi}(\btheta_0, \wh{\bfeta}) = O_p(N^{-\frac{1}{2}})$. 
Then, according to Lemma \ref{lem: E.1}, 
\[
\wh{\bPsi}(\bar{\btheta}, \wh{\bfeta}) = \wh{\bPsi}(\bar{\btheta}, {\bfeta}_0) + o_p(N^{-\frac{1}{2}}) = O_p(N^{-\frac{1}{2}}),
\]
which shows that \eqref{eq: claim: EL} holds with $\bar{\btheta} = \btheta_0$. 
Using the definition of the saddle point $(\wh{\btheta}, \bar{\lambda})$, the inequality \eqref{eq: E.2}, and the claim \eqref{eq: claim: EL} with , we have 
\begin{equation}
\begin{aligned}
     N^{-\xi}\norm{\wh{\bPsi}(\wh{\btheta}, \wh{\bfeta})} - C_3 N^{-2\xi} & \leq \aveiN\rho(\tilde{\lambda}\t \bPsi_i(\wh{\btheta}, \wh{\bfeta}))  \\ & \leq \aveiN\rho(\wh{\lambda}\t \bPsi_i(\wh{\btheta}, \wh{\bfeta}))  \\ & \leq  \sup_{\lambda \in \wh{\Lambda}_N({\btheta}_0)} \aveiN\rho(\lambda\t \bPsi_i({\btheta}_0, \wh{\bfeta})) = O_p(N^{-1}),
\end{aligned}
\label{eq: E.4}
\end{equation}
implying that $\norm{\wh{\bPsi}(\wh{\btheta}, \wh{\bfeta})} = O_p(N^{-1 + \xi}) + O_p(N^{-\xi}) =  O_p(N^{-\xi})$, since $\xi < 1/ 2$. Now, suppose $\epsilon_N$ is an arbitrary sequence that converges to $0$ and let $\tilde{\lambda} =  \epsilon_N \wh{\bPsi}(\wh{\btheta}, \wh{\bfeta})$, which implies $\tilde{\lambda} = o_p(N^{-\xi})$. Then, similar to \eqref{eq: E.4}, we have 
\begin{align}
    \tilde{\lambda}\t\norm{\wh{\bPsi}(\wh{\btheta}, \wh{\bfeta})} - C_3 \norm{\tilde{\lambda}}^2 = O_p(N^{-1}), \nn 
\end{align} 
which implies $  \epsilon_N (1- C_3 \epsilon_N) \norm{\wh{\bPsi}(\wh{\btheta}, \wh{\bfeta})}^2 = O_p(N^{-1})$. Since $1- C_3 \epsilon_N = O(1)$, we have $\epsilon_N \norm{\wh{\bPsi}(\wh{\btheta}, \wh{\bfeta})}^2 = O_p(N^{-1})$ for any sequence $\epsilon_N = o(1)$. Then it follows %from standard probability theories 
that $\norm{\wh{\bPsi}(\wh{\btheta}, \wh{\bfeta})} = O_p(N^{-\frac{1}{2}})$.  Similar to Lemma \ref{lem: E.1}, it implies that ${\wh{\bPsi}(\wh{\btheta}, {\bfeta}_0)}  = {\wh{\bPsi}(\wh{\btheta}, \wh{\bfeta})} + o_p(N^{-\frac{1}{2}}) = O_p(N^{-\frac{1}{2}})$. 

According to the uniform weak law of large numbers, 
\[
\sup_{\btheta\in\Theta} \norm{{\wh{\bPsi}({\btheta}, {\bfeta}_0)} - \bPsi(\btheta,{\bfeta}_0)} = o_p(1),
\]
which together with ${\wh{\bPsi}(\wh{\btheta}, {\bfeta}_0)}  = o_p(1)$
implies $\bPsi(\wh{\btheta}, {\bfeta}_0) = o_p(1)$. Since $ \bPsi({\btheta}, {\bfeta}_0)  = 0$ if and only if $\btheta = \btheta_0$ and $ \bPsi({\btheta}, {\bfeta}_0)$ is continuous with respect to $\btheta$, $\bPsi(\wh{\btheta}, {\bfeta}_0) = o_p(1)$ implies $\wh{\btheta} = \btheta_0 + o_p(1)$, which establishes the consistency of $\wh{\btheta}$.    
\end{proof}

\subsection{Proof of Theorem \ref{thm: asy dist}}

The saddle point $(\wh{\btheta}, \wh{\lambda})$ to \eqref{eq: E.1} satisfies $Q_{1,N}(\wh{\btheta}, \wh{\lambda}) = 0$ and $Q_{2,N}(\wh{\btheta}, \wh{\lambda}) = 0$, where 
\begin{align}
    Q_{1, N}(\wh{\btheta}, \wh{\lambda}) & =   \aveiN \frac{1}{1 + \wh{\lambda}\t \bPsi_i(\wh{\btheta}, \hetak)}\bPsi_i(\wh{\btheta}, \hetak) ,  ~~\text{and} \nn  \\ 
     Q_{2, N}(\wh{\btheta}, \wh{\lambda}) & =  \aveiN\frac{1}{1 + \wh{\lambda}\t \bPsi_i(\wh{\btheta}, \hetak)} \left(\frac{\partial \bPsi_i(\wh{\btheta}, \hetak)}{\partial \btheta} \right)\t \wh{\lambda}. \nn 
\end{align}
By Taylor expansion of $Q_{1,N}(\wh{\btheta}, \wh{\lambda}) = 0$ and $Q_{2,N}(\wh{\btheta}, \wh{\lambda}) = 0$ around $(\btheta_0, 0)$, we have 
\begin{equation*}
    \begin{aligned}
    0 & = Q_{1,n}(\btheta_0, 0) + \frac{\partial Q_{1,N}(\btheta_0,0)}{\partial \btheta} (\wh{\btheta} - \btheta_0) + \frac{\partial Q_{1,N}(\btheta_0,0)}{\partial \lambda} \wh{\lambda} + o_p(\delta_N), ~~\text{and}\\ 
     0 & = Q_{2,n}(\btheta_0, 0) + \frac{\partial Q_{2,N}(\btheta_0,0)}{\partial \btheta} (\wh{\btheta} - \btheta_0) + \frac{\partial Q_{2,N}(\btheta_0,0)}{\partial \lambda} \wh{\lambda} + o_p(\delta_N),
\end{aligned}
%\label{eq: Q-expan}
\end{equation*}
where $\delta_N = \norm{\wh{\btheta} - \btheta_0} + \norm{\wh{\lambda}}$, 
leading to 
\begin{align}
    \begin{pmatrix}\hat{\lambda} \\ 
    \wh{\btheta}-\btheta_0\end{pmatrix}
    =\bS_N^{-1}\begin{pmatrix}-Q_{1,N}(\btheta_0,0)+o_p(\delta_N)\\ -Q_{2,N}(\btheta_0,0)o_p(\delta_N)\end{pmatrix} = \bS_N^{-1}\begin{pmatrix}-Q_{1,N}(\btheta_0,0)+o_p(\delta_N)\\o_p(\delta_N)\end{pmatrix}, 
    \label{eq: lambda-theta-expan}
\end{align}
where
\begin{align*}
    \bS_N = 
\begin{pmatrix}
    \frac{\partial Q_{1,N}(\btheta_0,0)}{\partial \lambda} &  \frac{\partial Q_{1,N}(\btheta_0,0)}{\partial \btheta} \\ 
      \frac{\partial Q_{2,N}(\btheta_0,0)}{\partial \lambda} &  \frac{\partial Q_{2,N}(\btheta_0,0)}{\partial \btheta}
\end{pmatrix},
\end{align*}
and the partial derivatives are 
\begin{equation*}
\begin{aligned}
    \frac{\partial Q_{1,N}(\btheta_0,0)}{\partial \btheta} &=   \aveiN \frac{\partial \bPsi_i({\btheta}_0, \hetak)}{\partial \btheta}, ~~&\frac{\partial Q_{1,N}(\btheta_0,0)}{\partial \lambda}  = -  \aveiN  \bPsi_i({\btheta}_0, \hetak)^{\otimes 2}, \\ 
\frac{\partial Q_{2,N}(\btheta_0,0)}{\partial \btheta}& =  0, ~~&\frac{\partial Q_{2,N}(\btheta_0,0)}{\partial \lambda} =  \aveiN  \left( \frac{\partial \bPsi_i({\btheta}_0, \hetak)}{\partial \btheta}\right)\t. 
\end{aligned}
%\label{eq: Q-deriv}
\end{equation*}
Using the dominated convergence theorem, we can show that $\norm{\wh{\bbm} - \bbm_0} = o_p(1)$ implies $\norm{\partial\wh{\bbm}/ \partial \btheta - \partial{\bbm}_{0}/ \partial \btheta } = o_p(1)$. With the continuous mapping theorem and the law of large numbers, we have 
\begin{equation}
\begin{aligned}
      \frac{\partial Q_{1,N}(\btheta_0,0)}{\partial \btheta} &= \bGamma + o_p(1), ~~&\frac{\partial Q_{1,N}(\btheta_0,0)}{\partial \lambda}  = - \bOmega + o_p(1), \\ 
      \frac{\partial Q_{2,N}(\btheta_0,0)}{\partial \btheta}& =  0, ~~&\frac{\partial Q_{2,N}(\btheta_0,0)}{\partial \lambda} =\bGamma\t + o_p(1),
\end{aligned}
\label{eq: Q-deriv}
\end{equation}
where 
\begin{align}
    \bGamma = \E\left\{\frac{\partial \bPsi(\bW, \btheta_0, \bfeta_0)}{\partial \btheta} \right\}~~\text{and}~~\bOmega = \E\left\{ \bPsi(\bW, \btheta_0, \bfeta_0)^{\otimes 2}\right\}. \nn 
\end{align}
From Lemma \ref{lem: E.1}, we have 
\begin{align}
     Q_{1,N}(\btheta_0, 0) = \frac{1}{N}\sum_{i=1}^N \bPsi(\bW_i, \btheta_{0},\bfeta_{0}) + o_{p}(N^{-\frac{1}{2}}) = O_p(N^{-\frac{1}{2}}),  
     \label{eq: Q_1 expan}
\end{align}
where the last equality is due to the CLT. Combining \eqref{eq: lambda-theta-expan}, \eqref{eq: Q-deriv}, and \eqref{eq: Q_1 expan}, and using the continuous mapping theorem, we have 
\begin{align}
    \begin{pmatrix}\hat{\lambda} \\ 
    \wh{\btheta}-\btheta_0\end{pmatrix}
    =\left(
    \begin{pmatrix}
       -\bOmega & \bGamma \\ 
       \bGamma\t & 0 
    \end{pmatrix} 
    ^{-1} + o_p(1) \right)\begin{pmatrix} Q_{1,N}(\btheta_0, 0) +o_p(\delta_N)\\o_p(\delta_N)\end{pmatrix}, 
    \label{eq: lambda-theta}
\end{align}
assuming that the block matrix on the right-hand side is invertible. 
Since $\delta_N = \norm{\wh{\btheta} - \btheta_0} + \norm{\wh{\lambda}}$, we know that $\delta_N = O_P(N^{-\frac{1}{2}})$, which further implies that 
\[
\sqrt{N}(\wh{\btheta} - \btheta_0) = \left\{\bGamma\t \bOmega^{-1} \bGamma \right\}^{-1} \bGamma \bOmega^{-1} \sqrt{N} Q_{1,N}(\btheta_0, 0) + o_p(1) \indist \mathcal{N}(0, \left\{\bGamma\t \bOmega^{-1} \bGamma \right\}^{-1}), 
\]
which completes the proof of Theorem \ref{thm: asy dist}.

\subsection{Proof of Theorem \ref{thm: wilks}}

Since for every $\btheta \in \Theta$, the optimal empirical weight $p_i$ is given by 
\[
p_i = \frac{1}{N} \frac{1}{1 + \lambda(\btheta)\t \bPsi_i(\btheta, \hetak)}, ~~ i\in \cI_k, ~k = 1, \cdots, K,
\]
where $\lambda(\btheta)$ satisfies $Q_{1,N}(\btheta, \lambda(\btheta)) = 0$, 
the log EL statistics with a given $\btheta$ can be written as 
\[
\ell_N(\btheta) = \log\{ 1 + \lambda(\btheta)\t \bPsi_i(\btheta, \hetak) \}. 
\]
With $\btheta = \btheta_0$, solving $Q_{1,N}(\btheta_0, \lambda) = 0$ gives 
\[
\lambda(\btheta_0) = \Omega^{-1}Q_{1,N}(\btheta_0,0) + o_p(N^{-\frac{1}{2}}).
\]
Taking the expansion of $\ell_N(\btheta_0)$ leads to 
\begin{align}
    \ell_N(\btheta_0) = -\frac{N}{2} Q_{1,N}\t(\btheta_0,0) \Omega^{-1} Q_{1,N}(\btheta_0,0)+o_p(1). 
\end{align}
Using the characteristic of $\wh{\lambda}$ given in \eqref{eq: lambda-theta}, and expanding $\ell_N(\wh{\btheta})$ gives 
\begin{align}
      \ell_N(\btheta_0) = - \frac{N}{2} Q_{1,N}\t(\btheta_0,0) \bA Q_{1,N}(\btheta_0,0)+o_p(1),
\end{align}
where 
\[
\bA = -\bOmega^{-1}\{\bI + \bGamma (\bGamma\t \bOmega^{-1}\bGamma)^{-1} \bGamma\t \bOmega^{-1}\}.
\]
Therefore, $R_N(\btheta_0)$ is equivalent to 
\begin{align}
  R_N(\btheta_0) & = N    Q_{1,N}\t(\btheta_0,0) (\bA - \bOmega^{-1})  Q_{1,N}(\btheta_0,0) + o_p(1) \nn \\ 
  & =  N    Q_{1,N}\t(\btheta_0,0)  \bOmega^{-1} \bGamma  (\bGamma\t \bOmega^{-1}\bGamma)^{-1} \bGamma\t \bOmega^{-1} Q_{1,N}(\btheta_0,0) + o_p(1). \nn 
\end{align}
Note that $(-\bOmega)^{-\frac{1}{2}}\sqrt{N}Q_{1,N}(\btheta_0,0)$ weakly converges to a standard normal distribution,  and $$(-\bOmega)^{-\frac{1}{2}}\bGamma  (\bGamma\t \bOmega^{-1}\bGamma)^{-1} \bGamma\t(-\bOmega)^{-\frac{1}{2}}$$ is symmetric and idempotent with the trace equal to $r$. Hence, $ R_N(\btheta_0) \indist \chi^2_r$, which completes the proof of Theorem \ref{thm: wilks}.

\section{Proofs for Section \ref{sec: drw-theory}}

\subsection{Proof of Theorem \ref{thm: drw}}

\begin{lemma}\label{lemma: plug-in expectation}
Under Conditions \ref{con: dist}--\ref{con: hat-r},  
\begin{align}
\sqrt{N}\E\left\{ \frac{1-\delta}{1-p}\wh{r}(\bX)\bbm(\bX)  \right\} = \frac{1}{\sqrt{N}}\sumiN  \left\{ \frac{\delta_i}{p} \bbm(\bX_i) - \frac{1-\delta_i}{1-p} r_0(\bX_i) \bbm(\bX_i)  \right\} + o_p(1), 
\label{eq: linear rep of bias}
\end{align}    
where the expectation is taken with respect to $\bX$. 
\end{lemma}

\bigskip

Recall that the criterion function for the estimation of $r$ is defined as 
\[
\wh{L}_N(r) = \frac{1}{N}\sumiN \ell(\delta_i, \bX_i; r),
\]
where 
\begin{align}
    \ell(\delta, \bX; r) = \frac{1-\delta}{1-p}\ell_1(\bX; r) - \frac{\delta}{p}\ell_2(\bX; r). \nn 
\end{align}
\iffalse
Let $\wh{r}$ satisfy 
\begin{align}
    \wh{L}_N(\wh{r}) \leq \wh{L}_N(r) + O_p(\epsilon_N^2),~~~\forall r \in \cF_N,
\label{eq: L-obj}
\end{align}
where $\epsilon_N$ is a positive sequence satisfying $\epsilon_N = o(n^{-\frac{1}{2}})$. 
By Condition \ref{con: hat-r},(i) , we have 
\[
\norm{\wh{r} - r_0}_{L_2(P)} = O_p(\delta_N),
\]
where $\delta_N = o(n^{-\frac{1}{4}})$. 
\fi
The directional derivative of $\ell(\delta, \bX; r)$ with respect to $r$ in the direction $u \in L_2(P)$ is given by 
\begin{align}
    \frac{d}{d u} \ell(\delta, \bX; r)[u] := &\lim_{t \to 0} \frac{\ell(\delta, \bX; r+ t u) - \ell(\delta, \bX; r) }{t}  \nn \\ 
    = & \left\{ \frac{1-\delta}{1-p}\frac{\partial}{\partial r}\ell_1(\bX; r) - \frac{\delta}{p}\frac{\partial}{\partial r}\ell_2(\bX; r) \right\} u(\bX) \nn \\ 
   =: & ~\ell^{(1)}(\delta, \bX; r) u(\bX), ~~\text{say}.
    \label{eq: direction deriv}
\end{align}
%for any $u \in L_2(P)$, where the last equality is from Condition \ref{con: l1-l2}.(i). 
According to Condition \ref{con: l1-l2}. (ii), we have 
\[
\ell^{(1)}(\delta, \bX; r)  = \frac{1-\delta}{1-p}\frac{\partial}{\partial r}\ell_2(\bX; r) r(\bX) - \frac{\delta}{p}\frac{\partial}{\partial r}\ell_2(\bX; r).
\]
The first-order approximation error for $\ell(\delta, \bX; r_0)$ is denoted as 
\begin{align}
     e(\delta, \bX, r - r_0) =  \ell(\delta, \bX; r) - \ell(\delta, \bX; r_0)  -  \frac{d}{d u} \ell(\delta, \bX; r_0)[r - r_0].\nn 
\end{align}

With the above notations, for any $r \in \cF_N$, it holds that
\begin{align}
\wh{L}_N(r) =&  \wh{L}_N(r_0) + \{ \wh{L}_N(r) -  \wh{L}_N(r_0) \} \nn \\ 
= & \wh{L}_N(r_0) + \frac{1}{N} \sumiN \{ \ell(\delta_i, \bX_i; r) - \ell(\delta_i, \bX_i; r_0) \} \nn \\ 
= & \wh{L}_N(r_0) + \frac{1}{N} \sumiN \left\{ \frac{d}{d r} \ell(\delta_i, \bX_i; r_0) [r - r_0]  + e(\delta_i, \bX_i; r - r_0) \right\} \nn \\ 
= &   \wh{L}_N(r_0) +  \frac{1}{\sqrt{N}}\G_N \left( \frac{d}{d r} \ell(\delta_i, \bX_i; r_0) [r - r_0]\right) + \frac{1}{N} \sumiN e(\delta_i, \bX_i; r - r_0),
\label{eq: L-decom}
\end{align}
where the last equality is because 
\begin{align}
    \E\left\{\frac{d}{d r} \ell(\delta_i, \bX_i; r_0) [r - r_0] \right\} =  0. 
\end{align}

We will employ the Cramer-Wald device to establish \eqref{eq: linear rep of bias}. For any $\bv \in \mathbb{R}^p$ with $\norm{\bv} = 1$, we define $\tilde{m}_{\bv, \ell_2}(\bx) = \bbm(\bx)\t \bv \cdot (\partial \ell_2(\bx, r) / \partial r)^{-1}$. 
For any $r \in \mathcal{F}_N$,  let 
$$\bar{r}({r}, \epsilon_N) = (1- \epsilon_N) r + \epsilon_N(r_0+\tilde{m}_{\bv, \ell_2})$$ be a local alternative value around $r$ and 
$$\Pi_{\mathcal{F}_n}\bar{r}({r}, \epsilon_N) = (1- \epsilon_N) r + \epsilon_N(r_* + \tilde{m}_*),$$ 
where $r_* = \argmin_{r \in \cF_N} \norm{r - r_0}_{L_2(F)}$ and $\tilde{m}_* = \argmin_{m \in \cF_N} \norm{m - \tilde{m}_{\bv, \ell_2}}_{L_2(F)}$. In the light of Condition \ref{con: hat-r}, we have $\Pi_{\mathcal{F}_n}\bar{r}({r}, \epsilon_N) \in \cF_N$ and 
\begin{align}
    \sup_{r \in \cF_N}\norm{\Pi_{\cF_N} \bar{r}_{\bv, \ell_2}({r}, \epsilon_N) - \bar{r}_{\bv, \ell_2}({r}, \epsilon_N)}_{L_2(F)} = o( \epsilon_N  \cdot N^{-\frac{1}{4}}).
    \label{eq: approx bar-r}
\end{align}

By substituting $r$ with $\wh{r}$ and $\Pi_{\cF_n} \bar{r}(\wh{r}, \epsilon_N)$, respectively, we obtain 
\begin{align}
\wh{L}_N(\wh{r}) =  \wh{L}_N({r}_0) + \frac{1}{\sqrt{N}}\G_N \left( \frac{d}{d r} \ell(\delta_i, \bX_i; r_0) [\wh{r }- r_0]\right) + \frac{1}{N} \sumiN e(\delta_i, \bX_i; \wh{r} - r_0) 
\label{eq: L-hatr}
\end{align}
and 
\begin{align}
\wh{L}_N(\projr) =  &\wh{L}_N({r}_0) + \frac{1}{\sqrt{N}}\G_N \left( \frac{d}{d r} \ell(\delta_i, \bX_i; r_0) [\projr- r_0]\right) \nn \\ &+ \frac{1}{N} \sumiN e(\delta_i, \bX_i; \projr - r_0).  
\label{eq: L-projr}
\end{align}
Subtracting \eqref{eq: L-hatr} from \eqref{eq: L-projr} gives 
\begin{align}
\wh{L}_N(\wh{r}) = & \wh{L}_N(\projr) + {\frac{1}{\sqrt{N}}\G_N \left( \frac{d}{d r} \ell(\delta_i, \bX_i; r_0) [\wh{r} - \projr]\right) }\nn \\ 
& {+ \frac{1}{N} \sumiN \left\{e(\delta_i, \bX_i; \wh{r} - r_0) -   e(\delta_i, \bX_i; \projr - r_0)  \right\}. }
\label{eq:L-hatr-projr}
\end{align}
We will prove later in Subsection \ref {subsec: proof of diff-e} that 
\begin{align}
    & {\frac{1}{N} \sumiN \left\{e(\delta_i, \bX_i; \projr - r_0) - e(\delta_i, \bX_i; \wh{r} - r_0)   \right\}} \nn \\
{=}&~  {\epsilon_N(1- \epsilon_N) \E \left( \frac{1-\delta}{1-p} \{\wh{r}(\bX_i)- r_0(\bX) \}m_{\bv}(\bX_i)\right) + o_p\left(\frac{\epsilon_N}{\sqrt{N}} \right). }
\label{eq: diff-e}
\end{align}
By the definition of $\wh{r}$, we have 
\[
\wh{L}_N(\wh{r}) - \wh{L}_N(\projr) \leq O(\epsilon_N^2),
\]
which together with \eqref{eq:L-hatr-projr} and \eqref{eq: diff-e} yield 
\begin{align}
   & \frac{1}{\sqrt{N}} \G_N \left( \frac{d}{d r} \ell(\delta_i, \bX_i; r_0) [\wh{r} - \projr]\right)  \nn \\ & - \epsilon_N(1- \epsilon_N) \E \left( \frac{1-\delta}{1-p} \{\wh{r}(\bX_i)- r_0(\bX) \}m_{\bv}(\bX_i)\right) + o_p\left(\frac{\epsilon_N}{\sqrt{N}}\right) \leq O(\epsilon_N^2). 
   \label{eq:10}
\end{align}
For the term $\G_N \left( \frac{d}{d r} \ell(\delta_i, \bX_i; r_0) [\wh{r} - \projr]\right) $, we have 
\begin{align}
    & \G_N \left( \frac{d}{d r} \ell(\delta_i, \bX_i; r_0) [\wh{r} - \projr]\right)  \nn \\ 
= & \G_N \left( \frac{d}{d r} \ell(\delta_i, \bX_i; r_0) [\wh{r} - \barr]\right) + \G_N \left( \frac{d}{d r} \ell(\delta_i, \bX_i; r_0) [\barr - \projr]\right) \nn \\ 
= & \G_N \left( \frac{d}{d r} \ell(\delta_i, \bX_i; r_0) [\wh{r} - \barr]\right)  + o_p(\epsilon_N)% \red{O_p(\sqrt{N}\epsilon_N^2)~ (or ~o_p(\epsilon_N)?)}
,\nn 
\end{align}
where the last equality is due to \eqref{eq: approx bar-r} and the Chebyshev inequality. By the definition of $\barr$, we have 
\begin{align}
   & \G_N \left( \frac{d}{d r} \ell(\delta_i, \bX_i; r_0) [\wh{r} - \barr]\right) \nn \\ = & \epsilon_N \G_N\left( \frac{d}{d r} \ell(\delta_i, \bX_i; r_0) [\wh{r} - r_0]\right)  - \epsilon_N \G_N\left( \frac{d}{d r} \ell(\delta_i, \bX_i; r_0) [\tilde{m}_{\bv, \ell}]\right). 
\end{align}
We now show that $\G_N\left( \frac{d}{d r} \ell(\delta_i, \bX_i; r_0) [\wh{r} - r_0]\right) = o_p(1)$. By \eqref{eq: direction deriv}, 
\[
 \frac{d}{d r} \ell(\delta_i, \bX_i; r_0) [\wh{r} - r_0] = \ell^{(1)}(\delta_i, \bX_i; r_0)\{\wh{r}(\bX_i) - r_0(\bX_i) \}. 
\]
Let 
\[
\tilde{\cF}_N = \left\{ \ell^{(1)}(\delta, \bx; r_0)\{r(\bx) - r_0(\bx) \}:~r \in \cF_N, \norm{r - r_0}_{L_2(F)} \leq \delta_N  \right\},
\]
then it is evident that 
\[
\log N_{[\ ]}(\epsilon, \tilde{\cF}_N,  L_2(F)) \lesssim \log  N_{[\ ]}(\epsilon, {\cF}_N,  L_2(F))
\]
for any $\epsilon > 0$. Therefore, the bracketing number of $\tilde{F}_N$ satisfies 
\begin{align}
    J_{[\ ]}(\delta_N, \tilde{\cF}_N,  L_2(F)) &= \int_0^{\delta_N}\sqrt{1 + \log  N_{[\ ]}(\epsilon, \tilde{\cF}_N,  L_2(F))} d\epsilon  \nn \\ 
&\lesssim \int_0^{\delta_N}\sqrt{1 + \log  N_{[\ ]}(\epsilon, {\cF}_N,  L_2(F))} d\epsilon  \nn \\ 
&= J_{[\ ]}(\delta_N, {\cF}_N,  L_2(F)) = o(1)\nn 
\end{align}
by Condition \ref{con: hat-r} (iii). Also, for every $f \in \tilde{F}_N$, it holds that $\norm{f}_\infty = O(1)$ and $\norm{f}_{L_2(F)} = O(\delta_N)$. By applying Lemma 3.4.2 of \cite{van1996weak}, we have 
\begin{align}
    \E\norm{\G_N}_{\tilde{F}_N} \lesssim J_{[\ ]}(\delta_N, \tilde{\cF}_N,  L_2(F)) \left(1 + \frac{J_{[\ ]}(\delta_N, \tilde{\cF}_N,  L_2(F))}{\delta_N^2 \sqrt{N}} O(1) \right) = o(1),\nn 
\end{align}
which, by the Markov inequality, implies that 
\begin{align}
\sup_{r\in {\cF}_N} \G_N\left(\ell^{(1)}(\delta, \bx; r_0)\{r(\bx) - r_0(\bx) \} \right) = o_p(1),
\label{eq: sec}
\end{align}
meaning that 
\begin{align}
   \epsilon_N \G_N\left( \frac{d}{d r} \ell(\delta_i, \bX_i; r_0) [\wh{r} - r_0]\right)  = o_p(\epsilon_N).  \nn 
\end{align}

In addition, 
plugging $\tilde{m}_{\bv, \ell}(\bX_i) = m_{\bv}(\bX_i)  \cdot \{ \frac{\partial}{\partial r}\ell_2(\bX_i, r_0)\}^{-1}$ into the directional derivative specified in \eqref{eq: direction deriv} gives 
\begin{align}
- \G_N\left( \frac{d}{d r} \ell(\delta_i, \bX_i; r_0) [\tilde{m}_{\bv, \ell}]\right) = \frac{1}{\sqrt{N}} \sumiN 
 \left\{ \frac{\delta_i}{p} m_{\bv}(\bX_i) - \frac{1-\delta_i}{1-p} r_0(\bX_i) m_{\bv}(\bX_i)  \right\}.\nn 
\end{align}

Combining the above results gives 
\begin{align}
    & {\G_N \left( \frac{d}{d r} \ell(\delta_i, \bX_i; r_0) [\wh{r} - \projr]\right)} \nn \\ {=} & {\frac{\epsilon_N}{\sqrt{N}} \sumiN 
 \left\{ \frac{\delta_i}{p} m_{\bv}(\bX_i) - \frac{1-\delta_i}{1-p} r_0(\bX_i) m_{\bv}(\bX_i)  \right\} + o_p(\epsilon_N)}.  \nn  
\end{align}
Therefore, multiplying the both sides of \eqref{eq:10} by $\sqrt{N} / \epsilon_N$ leads to 
\begin{align}
  & \frac{1}{\sqrt{N}} \sumiN 
 \left\{ \frac{\delta_i}{p} m_{\bv}(\bX_i) - \frac{1-\delta_i}{1-p} r_0(\bX_i) m_{\bv}(\bX_i)  \right\} + o_p(\epsilon_N) \nn \\ & -\sqrt{N}(1- \epsilon_N) \E \left( \frac{1-\delta}{1-p} \{\wh{r}(\bX_i)- r_0(\bX) \}m_{\bv}(\bX_i)\right) = o_p(1) + O_p\left(\frac{\epsilon_N}{\sqrt{N}} \right) = o_p(1), \nn 
\end{align}
which completes the proof of Lemma \ref{lemma: plug-in expectation}.

\subsection{Proof of \eqref{eq: diff-e}} 
\label{subsec: proof of diff-e}

First, for any candidate $r$ we can decompose $e(\delta, \bX, r - r_0)$ as 
\begin{align}
    & e(\delta, \bX, r - r_0)  \nn \\
= & \ell(\delta, \bX; r) - \ell(\delta, \bX; r_0)  -  \frac{d}{d u} \ell(\delta, \bX; r_0)[r - r_0] \nn \\ 
= & \frac{1}{2} \left\{ \frac{1-\delta}{1-p}\frac{\partial^2}{\partial r^2}\ell_1(\bX; r_0) - \frac{\delta}{p}\frac{\partial^2}{\partial r^2}\ell_2(\bX; r_0) \right\} \{r(\bX) - r_0(\bX) \}^2 + R(\delta,  \bX, r),
\label{eq: def-e}
\end{align} 
where the remainder term $R(\delta,  \bX, r)$ is 
\[
R(\delta,  \bX, r) = \frac{1}{2} \int_{r_0(\bX)}^{r(\bX)} \left\{ \frac{1-\delta}{1-p}\frac{\partial^3}{\partial r^3}\ell_1(\bX; t) - \frac{\delta}{p}\frac{\partial^3}{\partial r^3}\ell_2(\bX; t) \right\} \{r(\bX) - t \}^2  d t ,
\]
and the last equality of \eqref{eq: def-e} is due to the following Taylor's theorem 
\[
f(b) = f(a) + f'(a) (b-a) + \frac{f''(a)}{2}(b-a)^2 + \int_a^b \frac{f'''(t)}{2}(b-t)^2 dt . 
\]
Let 
\[
\ell^{(2)}(\delta, \bX) :=\frac{1-\delta}{1-p}\frac{\partial^2}{\partial r^2}\ell_1(\bX; r_0) - \frac{\delta}{p}\frac{\partial^2}{\partial r^2}\ell_2(\bX; r_0).
\]
Then, according to Condition \ref{con: l1-l2}.(i), we have 
\begin{align}
    &\frac{\partial}{\partial r} \ell_1(\bX; r_0) = r_0(\bX)  \frac{\partial}{\partial r} \ell_2(\bX; r_0), \nn \\ 
    & \frac{\partial^2}{\partial r^2} \ell_1(\bX; r_0) = r_0(\bX)  \frac{\partial^2}{\partial r^2} \ell_2(\bX; r_0) + \frac{\partial}{\partial r} \ell_2(\bX; r_0),\nn 
\end{align}
which implies that 
\begin{align}
    \ell^{(2)}(\delta, \bX) = \frac{1-\delta}{1-p}\left\{  r_0(\bX)  \frac{\partial^2}{\partial r^2} \ell_2(\bX; r_0) + \frac{\partial}{\partial r} \ell_2(\bX; r_0) \right\}- \frac{\delta}{p}\frac{\partial^2}{\partial r^2}\ell_2(\bX; r_0).
\label{eq: l''}
\end{align}

The last term in \eqref{eq:L-hatr-projr} can be written as 
\begin{align}
&\frac{1}{N} \sumiN \left\{e(\delta_i, \bX_i; \projr - r_0) - e(\delta_i, \bX_i; \wh{r} - r_0)   \right\} \nn \\ 
= &  \frac{1}{2N} \sumiN  \left\{ \frac{1-\delta}{1-p}\frac{\partial^2}{\partial r^2}\ell_1(\bX; r_0) - \frac{\delta}{p}\frac{\partial^2}{\partial r^2}\ell_2(\bX; r_0) \right\} \{\projr(\bX_i) - r_0(\bX_i) \}^2   \nn \\ 
& -\frac{1}{2N} \sumiN  \left\{ \frac{1-\delta}{1-p}\frac{\partial^2}{\partial r^2}\ell_1(\bX; r_0) - \frac{\delta}{p}\frac{\partial^2}{\partial r^2}\ell_2(\bX; r_0) \right\} \{\wh{r}(\bX_i) - r_0(\bX_i) \}^2   \nn \\ 
&+   \frac{1}{N} \sumiN  \{ R(\delta_i, \bX_i, \projr) - R(\delta_i, \bX_i, \wh{r}) \} \nn \\ 
=: & E_{1,N} + E_{2,N} + E_{3,N}, ~~~\text{say}. \nn 
\end{align}
For the term $\{\projr(\bX_i) - r_0(\bX_i) \}^2$, we have 
\begin{align}
&\{\projr(\bX_i) - r_0(\bX_i) \}^2 \nn \\ 
= & \{\projr(\bX_i)  - \bar{r}_{\bv, \ell_2}(\wh{r} , \epsilon_N)(\bX_i) +  \bar{r}_{\bv, \ell_2}(\wh{r} , \epsilon_N)(\bX_i)- r_0(\bX_i)\}^2 \nn \\ 
= & \{\projr(\bX_i)  - \bar{r}_{\bv, \ell_2}(\wh{r} , \epsilon_N)(\bX_i) + (1- \epsilon_N)(\wh{r}(\bX_i) - r_0(\bX_i) ) + \epsilon_N \tilde{m}_{\bv, \ell_2}(\bX_i)\}^2 \nn \\ 
= & \{\projr(\bX_i)  - \bar{r}_{\bv, \ell_2}(\wh{r} , \epsilon_N)(\bX_i) \}^2 + (1- \epsilon_N)^2\{ \wh{r}(\bX_i) - r_0(\bX_i) \} ^2 + \epsilon_N^2 \tilde{m}_{\bv, \ell_2}^2(\bX_i) \nn \\ 
& + 2 (1-\epsilon_N) \{\projr(\bX_i)  - \bar{r}_{\bv, \ell_2}(\wh{r} , \epsilon_N)(\bX_i) \}\{ \wh{r}(\bX_i) - r_0(\bX_i) \} \nn \\ 
& + 2 \epsilon_N \{\projr(\bX_i)  - \bar{r}_{\bv, \ell_2}(\wh{r} , \epsilon_N)(\bX_i) \} \tilde{m}_{\bv, \ell_2} (\bX_i) \nn \\ 
& + {2(1-\epsilon_N) \epsilon_N \{ \wh{r}(\bX_i) - r_0(\bX_i) \}\tilde{m}_{\bv, \ell_2}(\bX_i)}. 
\label{eq: projr-r0}
\end{align}

Using \eqref{eq: projr-r0}, we can decompose $E_{1,N} + E_{2,N} $ as 
\begin{align}
&E_{1, N} + E_{2,N} \nn \\ 
=& \frac{1}{2N} \sumiN \ell^{(2)}(\delta_i, \bX_i) [ \{\projr(\bX_i) - r_0(\bX_i) \}^2  - \{\wh{r}(\bX_i) - r_0(\bX_i) \}^2 ] \nn \\ 
=& \frac{1}{2N} \sumiN \ell^{(2)}(\delta_i, \bX_i)\{\projr(\bX_i)  - \bar{r}_{\bv, \ell_2}(\wh{r} , \epsilon_N)(\bX_i) \}^2 \nn \\ 
& + \frac{(1- \epsilon_N)^2 - 1 }{2N} \sumiN \ell^{(2)}(\delta_i, \bX_i) \{ \wh{r}(\bX_i) - r_0(\bX_i) \} ^2   + \frac{\epsilon_N^2}{2N}\ell^{(2)}(\delta_i, \bX_i)  \tilde{m}_{\bv, \ell_2}^2(\bX_i) \nn \\ 
& + \frac{1-\epsilon_N}{N} \sumiN \ell^{(2)}(\delta_i, \bX_i)\{\projr(\bX_i)  - \bar{r}_{\bv, \ell_2}(\wh{r} , \epsilon_N)(\bX_i) \}\{ \wh{r}(\bX_i) - r_0(\bX_i) \} \nn \\  
& + \frac{\epsilon_N}{N} \sumiN \ell^{(2)}(\delta_i, \bX_i)\{\projr(\bX_i)  - \bar{r}_{\bv, \ell_2}(\wh{r} , \epsilon_N)(\bX_i) \} \tilde{m}_{\bv, \ell_2}(\bX_i) \nn \\  
& + \frac{\epsilon_N(1- \epsilon_N)}{N} \sumiN \ell^{(2)}(\delta_i, \bX_i) \{ \wh{r}(\bX_i) - r_0(\bX_i) \}\tilde{m}_{\bv, \ell_2}(\bX_i) \nn \\ 
= & \frac{1}{2} \E[\ell^{(2)}(\delta_i, \bX_i)\{\projr(\bX_i)  - \bar{r}_{\bv, \ell_2}(\wh{r} , \epsilon_N)(\bX_i) \}^2  ] \{ 1+ o_p(1)\} \nn \\ 
& + \frac{\epsilon_N^2 - 2 \epsilon_N}{2 }\E[\ell^{(2)}(\delta_i, \bX_i) \{ \wh{r}(\bX_i) - r_0(\bX_i) \} ^2] \{ 1+ o_p(1)\} + \frac{\epsilon_N^2}{2} \E\{ \ell^{(2)}(\delta_i, \bX_i)  \tilde{m}_{\bv, \ell_2}^2(\bX_i)\} \{ 1+ o_p(1)\} \nn \\ 
& + (1-\epsilon_N)\E[\ell^{(2)}(\delta_i, \bX_i)\{\projr(\bX_i)  - \bar{r}_{\bv, \ell_2}(\wh{r} , \epsilon_N)(\bX_i) \}\{ \wh{r}(\bX_i) - r_0(\bX_i) \} ]\{ 1+ o_p(1)\} \nn \\ 
& + \epsilon_N \E\{ \ell^{(2)}(\delta_i, \bX_i) \{\projr(\bX_i)  - \bar{r}_{\bv, \ell_2}(\wh{r} , \epsilon_N)(\bX_i) \} \tilde{m}_{\bv, \ell_2}(\bX_i) \} \nn \\ 
& + \frac{\epsilon_N(1- \epsilon_N)}{N} \sumiN \ell^{(2)}(\delta_i, \bX_i) \{ \wh{r}(\bX_i) - r_0(\bX_i) \}\tilde{m}_{\bv, \ell_2}(\bX_i) \nn \\ 
\leq & O_p(\epsilon_N^2 \delta_N^2) + O_p(\epsilon_N \delta_N^2) + O_p(\epsilon_N^2) + O_p(\epsilon_N \delta^2_N) + O_p(\epsilon_N^2 \delta_N) \nn \\ 
& + \frac{\epsilon_N(1- \epsilon_N)}{N} \sumiN \ell^{(2)}(\delta_i, \bX_i) \{ \wh{r}(\bX_i) - r_0(\bX_i) \}\tilde{m}_{\bv, \ell_2}(\bX_i), 
\label{eq: E1+E2-1}
\end{align}
where the expectations are taken with respect to $(\delta_i, \bX_i)$, and the last equality is by the uniform boundness of $\ell^{(2)}(\delta, \bX)$, the approximation error in \eqref{eq: approx bar-r}, 
and the bounded moment of $\norm{\tilde{m}_{\bv, \ell_2}}^2$. 
%conditional on $\norm{\wh{r} - r_0}_{L_2(P)} = O(\delta_N)$ we have 
%\begin{align}
%  \E[\ell^{(2)}(\delta_i, \bX_i)\{\projr(\bX_i)  - \bar{r}_{\bv, \ell_2}(\wh{r} , \epsilon_N)(\bX_i) \}^2  ]  &= O_p(\epsilon_N^2 \delta_N^2), \nn \\ 
%   \frac{\epsilon_N^2 - 2 \epsilon_N}{2 }\E[\ell^{(2)}(\delta_i, \bX_i) \{ \wh{r}(\bX_i) - r_0(\bX_i) \} ^2] &=  O_p(\epsilon_N \delta_N^2), \nn \\ 
%  \frac{\epsilon_N^2}{2} \E\{ \ell^{(2)}(\delta_i, \bX_i)  \tilde{m}_{\bv, \ell_2}^2(\bX_i)\}  &= O_p(\epsilon_N^2),   \nn \\ 
%  (1-\epsilon_N)\E[\ell^{(2)}(\delta_i, \bX_i)\{\projr(\bX_i)  - \bar{r}_{\bv, \ell_2}(\wh{r} , \epsilon_N)(\bX_i) \}\{ \wh{r}(\bX_i) - r_0(\bX_i) \} &= O_p(\epsilon_N \delta^2_N),\nn \\
%      \epsilon_N \E\{ \ell^{(2)}(\delta_i, \bX_i) \{\projr(\bX_i)  - \bar{r}_{\bv, \ell_2}(\wh{r} , \epsilon_N)(\bX_i) \} \tilde{m}_{\bv, \ell_2}(\bX_i) \}  &= O_p(\epsilon_N^2 \delta_N)
%\end{align}
For the last term in \eqref{eq: E1+E2-1}, we note that
\begin{align}
& \frac{1}{N} \sumiN \ell^{(2)}(\delta_i, \bX_i) \{ \wh{r}(\bX_i) - r_0(\bX_i) \}\tilde{m}_{\bv, \ell_2}(\bX_i) \nn \\= & 
\frac{1}{\sqrt{N}} \G_N \left(\ell^{(2)}(\delta_i, \bX_i) \{ \wh{r}(\bX_i) - r_0(\bX_i) \}\tilde{m}_{\bv, \ell_2}(\bX_i) \right) \nn  \\ 
&+ \E\left( \ell^{(2)}(\delta_i, \bX_i) \{ \wh{r}(\bX_i) - r_0(\bX_i) \}\tilde{m}_{\bv, \ell_2}(\bX_i) \right),
\label{eq: ave-l2}
\end{align}
where the expectation is taken with respect to $(\delta_i, \bX_i)$. 
By the stochastic equicontinuity which can be derived with the similar arguments as for \eqref{eq: sec}, we can obtain 
\begin{align}
     \G_N \left(\ell^{(2)}(\delta_i, \bX_i) \{ \wh{r}(\bX_i) - r_0(\bX_i) \}\tilde{m}_{\bv, \ell_2}(\bX_i) \right) = o_p(1).
    \label{eq: ep-l2}
\end{align}
In the light of \eqref{eq: l''} and $\tilde{m}_{\bv, \ell_2}(\bX_i) = m_{\bv}(\bX_i)\cdot \{ \frac{\partial}{\partial r}\ell_2(\bX_i, r_0)\}^{-1}$, the expectation term can be written as 
\begin{align}
   &\E\left( \ell^{(2)}(\delta_i, \bX_i) \{ \wh{r}(\bX_i) - r_0(\bX_i) \}\tilde{m}_{\bv, \ell_2}(\bX_i) \right) \nn \\ 
   =& \E\left( \frac{1-\delta}{1-p}  \left\{ r_0(\bX) \frac{\partial^2}{\partial r^2} \ell_2(\bX; r_0) + \frac{\partial}{\partial r} \ell_2(\bX; r_0) \right\} 
  \{ \wh{r}(\bX_i) - r_0(\bX_i) \} m_{\bv}(\bX_i)\cdot \{ \frac{\partial}{\partial r}\ell_2(\bX_i, r_0)\}^{-1} \right)  \nn \\ 
   & -\E \left\{ \frac{\delta}{p}\frac{\partial^2}{\partial r^2}\ell_2(\bX; r_0)  \{ \wh{r}(\bX_i) - r_0(\bX_i) \} m_{\bv}(\bX_i)\cdot \{ \frac{\partial}{\partial r}\ell_2(\bX_i, r_0)\}^{-1} \right\} \nn \\ 
   =& \E \left( \frac{1-\delta}{1-p} \{\wh{r}(\bX_i)- r_0(\bX) \}m_{\bv}(\bX_i)\right),
   \label{eq: mean-l2}
\end{align}
where the last equality is due to $\E\{(1-\delta) r_0(\bX) f(\bX) \} = \E\{\delta f(\bX)  \}$ for any $f(\bX)$. 
Combining \eqref{eq: E1+E2-1}, \eqref{eq: ave-l2}, \eqref{eq: ep-l2}, and \eqref{eq: mean-l2}, and taking the convergence rate $\delta_N = o_p(N^{-\frac{1}{4}})$, we obtain 
\begin{align}
    E_{1,N} + E_{2,N} = 
    \epsilon_N(1- \epsilon_N) \E \left( \frac{1-\delta}{1-p} \{\wh{r}(\bX_i)- r_0(\bX) \}m_{\bv}(\bX_i)\right) + o_p\left(\frac{\epsilon_N}{\sqrt{N}} \right).
    \label{eq: E1+E2}
\end{align}

For the term $E_{3,N}$, we let 
\[
\ell^{(3)}(\delta, \bX; t) = \frac{1-\delta}{1-p}\frac{\partial^3}{\partial r^3}\ell_1(\bX; t) - \frac{\delta}{p}\frac{\partial^3}{\partial r^3}\ell_2(\bX; t). 
\]
Due to $\frac{\partial }{\partial r} \ell_1(\bX,t) = t \cdot \frac{\partial }{\partial r} \ell_2(\bX,t)$ imposed in Condition \ref{con: l1-l2}, we have 
\begin{align}
\ell^{(3)}(\delta, \bX; t) =  \frac{1-\delta}{1-p}\left\{t \cdot \frac{\partial^3}{\partial r^3}\ell_2(\bX; t) + \frac{\partial^2}{\partial r^2}\ell_2(\bX; t)  + \frac{\partial}{\partial r}\ell_2(\bX; t) \right\} - \frac{\delta}{p} \frac{\partial^3}{\partial r^3}\ell_2(\bX; t),
\end{align}
which is uniformly bounded by some positive constant $c_{\ell}$ according to Condition \ref{con: l1-l2}.(ii).

then $E_{3,N}$ can be decomposed as 
\begin{align}
E_{3,N} = & \frac{1}{N} \sumiN  \{ R(\delta_i, \bX_i, \projr) - R(\delta_i, \bX_i, \wh{r}) \} \nn \\ 
= & \frac{1}{2N} \sumiN  \int_{r_0(\bX_i)}^{\projr} \ell^{(3)}(\delta_i, \bX_i;t)  \{\projr - t \}^2  d t  \nn \\
& -  \frac{1}{2N} \sumiN \int_{r_0(\bX_i)}^{\wh{r}(\bX_i)}
\ell^{(3)}(\delta_i, \bX_i;t) \{\wh{r}(\bX_i) - t \}^2  d t \nn  \\ 
= & \frac{1}{2N} \sumiN \int_{\wh{r}(\bX_i)}^{\projr} \ell^{(3)}(\delta_i, \bX_i; t) \{\projr - t \}^2 dt \nn \\ 
& - \frac{1}{2N} \sumiN \int_{r_0(\bX_i)}^{\wh{r}(\bX_i)} \ell^{(3)}(\delta_i, \bX_i; t)[ \{\wh{r}(\bX_i) - t \}^2  - \{\projr - t \}^2 ] dt \nn \\ 
=: & D_{1,N} + D_{2,N}, ~~~\text{say.} \nn 
\end{align}

For the term $D_{1,N}$, we have 
\begin{align}
 2|D_{1,N}| & = \frac{1}{N} \abs{ \sumiN \int_{\wh{r}(\bX_i)}^{\projr} \ell^{(3)}(\delta_i, \bX_i; t) \{\projr - t \}^2 dt} \nn \\ 
 & \leq \frac{c_{\ell}}{N} \sumiN \abs{\int_{\wh{r}(\bX_i)}^{\projr}  \{\projr - t \}^2 dt} \nn \\ 
 & =  \frac{c_{\ell}}{N} \sumiN  (1-s_i)\abs{\{\projr -   \wh{r}(\bX_i) \}^3} ~~~(\text{for some } s_i \in (0,1)) \nn \\ 
 & \leq \frac{c_{\ell}}{N} \sumiN  \abs{\projr -   \wh{r}(\bX_i)}^3 \nn  \\ 
 & \leq \frac{2 c_{\ell}}{N}  \sumiN  \{ \abs{\projr - \barr}^3 + \abs{\barr - \wh{r}(\bX_i)}^3 \}, \nn %\\ 
 %&~~~~~+ 3 \abs{\projr - \barr}^2\abs{\barr - \wh{r}(\bX_i)} \nn \\ 
%&~~~~~ + 3\abs{\projr - \barr}\abs{\barr - \wh{r}(\bX_i)}^2 \}, \nn
\end{align}
where the first inequality is from the uniform boundness of $\ell^{(3)}(\delta_i, \bX_i; t)$, the second equality is by applying the mean value theorem, and the last inequality is from the inequality $(a+b)^3 \leq 2 (a^3 + b^3)$ for any positive $a$ and $b$. From \eqref{eq: approx bar-r} it can be easily derived that $\max_{1\leq i \leq N}\abs{\projr - \barr} = o_p(1)$.  For the term $\abs{\barr - \wh{r}(\bX_i)}$, we have 
\begin{align}
& \aveiN \abs{\barr - \wh{r}(\bX_i)} = \epsilon_N \aveiN \{\wh{r}(\bX_i) - r_0(\bX_i)- \tilde{m}_{\bv, \ell_2}(\bX_i) \} = O_p(\epsilon_N),
\label{eq: ave bar-hatr}
\\ 
& \aveiN \abs{\barr - \wh{r}(\bX_i)}^2 = \epsilon_N^2 \aveiN \{\wh{r}(\bX_i) - r_0(\bX_i)- \tilde{m}_{\bv, \ell_2}(\bX_i) \}^2 = O_p(\epsilon_N^2), 
\label{eq: ave bar-hatr^2}
\end{align}
Using Lemma 2 of \cite{owen1990}, it holds that $\max_{1 \leq i \leq N}|\tilde{m}_{\bv, \ell_2}(\bX_i)| = o_p(\sqrt{N})$, which together with the uniform boundness of $\wh{r}$ and $r_0$ and $\epsilon_N = o_p(N^{-\frac{1}{2}})$ imply that 
\begin{align}
    \max_{1 \leq i \leq N}\abs{\barr - \wh{r}(\bX_i)} & = \epsilon_N \max_{1 \leq i \leq N} \abs{\wh{r}(\bX_i) - r_0(\bX_i)- \tilde{m}_{\bv, \ell_2}(\bX_i)}  = o_p(1).
\label{eq: max bar-hatr}
\end{align}
Therefore, $|D_{1,N}|$ can be bounded by 
\begin{align}
    |D_{1,N}|\leq o_p(\epsilon_N^2\delta_N^2) + %o_p(\epsilon_N^3\log(N)) + o_p(\epsilon_N^2\delta_N^2\log(N)) +
    o_p(\epsilon_N^2) =o_p\left( \frac{\epsilon_N}{\sqrt{N}}\right),
\end{align}
where the equality is due to  $\epsilon_N = o(N^{-\frac{1}{2}})$ and $\delta_N = o(N^{-\frac{1}{4}})$.

For the term $D_{2,N}$, we have 
\begin{align}
    2|D_{2,N}| & = \frac{1}{N}\abs{\sumiN \int_{r_0(\bX_i)}^{\wh{r}(\bX_i)} \ell^{(3)}(\delta_i, \bX_i; t)[ \{\wh{r}(\bX_i) - t \}^2  - \{\projr - t \}^2 ] dt}  \nn \\ 
  & =   \frac{1}{N}\abs{\sumiN \int_{r_0(\bX_i)}^{\wh{r}(\bX_i)} \ell^{(3)}(\delta_i, \bX_i; t)[ \{\wh{r}(\bX_i) - \projr \}  \{\wh{r}(\bX_i) + \projr - 2t \} ] dt}  \nn \\ 
  & \leq  \frac{c_{\ell}}{N} \sumiN \int_{r_0(\bX_i)}^{\wh{r}(\bX_i)}  \abs{\wh{r}(\bX_i) - \projr }  \abs{\wh{r}(\bX_i) + \projr - 2t } dt \nn \\ 
  & \leq \frac{c_{\ell}}{N} \sumiN  \left\{ \abs{\wh{r}(\bX_i) - r_0(\bX_i)} \abs{\wh{r}(\bX_i) - \projr } \right. \nn \\ 
  & ~~~~~~~~~~\left.\cdot \abs{\wh{r}(\bX_i) + \projr  - 2\{s_i \wh{r}(\bX_i) + (1-s_i) r_0(\bX_i) \}} \right\} ~~~(\text{for some } s_i \in (0,1)) \nn \\ 
  & =  \frac{c_{\ell}}{N} \sumiN  \left\{ \abs{\wh{r}(\bX_i) - r_0(\bX_i)} \abs{\wh{r}(\bX_i) - \projr } \right. \nn \\ 
  & ~~~~~~~~~~\left.\cdot \abs{\projr  - \wh{r}(\bX_i) +   2(1-s_i) \{\wh{r}(\bX_i) - r_0(\bX_i) \}} \right\} \nn \\ 
  & \leq \frac{c_{\ell}}{N} \sumiN  \left\{ \abs{\wh{r}(\bX_i) - r_0(\bX_i)} (\abs{ \projr - \barr } + \abs{\barr - \wh{r}(\bX_i)} )\right. \nn \\ 
  & ~~~~~~~~~~\left.\cdot  (\abs{ \projr - \barr } + \abs{\barr - \wh{r}(\bX_i)} +   2 \abs{\wh{r}(\bX_i) - r_0(\bX_i)} )  \right\} \nn \\ 
  & = \frac{c_{\ell}}{N} \sumiN \abs{\wh{r}(\bX_i) - r_0(\bX_i)} \abs{ \projr - \barr }^2 \nn \\ 
      & ~~~+\frac{c_{\ell}}{N} \sumiN \abs{\wh{r}(\bX_i) - r_0(\bX_i)} \abs{ \projr - \barr }  \abs{\barr - \wh{r}(\bX_i)} \nn \\ 
        & ~~~+\frac{2 c_{\ell}}{N} \sumiN \abs{\wh{r}(\bX_i) - r_0(\bX_i)}^2 \abs{ \projr - \barr }  \nn \\
      & ~~~+\frac{c_{\ell}}{N} \sumiN \abs{\wh{r}(\bX_i) - r_0(\bX_i)} \abs{\barr - \wh{r}(\bX_i)} \abs{ \projr - \barr } \nn \\ 
       & ~~~+\frac{c_{\ell}}{N} \sumiN \abs{\wh{r}(\bX_i) - r_0(\bX_i)} \abs{\barr - \wh{r}(\bX_i)}^2 \nn \\ 
        & ~~~+\frac{2 c_{\ell}}{N} \sumiN \abs{\wh{r}(\bX_i) - r_0(\bX_i)}^2 \abs{\barr - \wh{r}(\bX_i)}, 
    \label{eq: D2N-1}
\end{align}
where the first inequality is from the uniform boundness of $\ell^{(3)}(\delta_i, \bX_i; t)$ and the second inequality is by applying the mean value theorem. 
By the  uniform boundness of $\wh{r}$ and $r_0$, the approximation error in \eqref{eq: approx bar-r}, \eqref{eq: ave bar-hatr^2}, $\norm{\wh{r} - r_0}_{L_2(P)} = O_p(\delta_N)$, and the Cauchy-Schwarz inequality, we can obtain
\begin{align}
& \aveiN \abs{\wh{r}(\bX_i) - r_0(\bX_i)} \abs{ \projr - \barr }^2 = O_p(\epsilon_N^2 \delta_N^2), \nn \\ 
& \aveiN \abs{\wh{r}(\bX_i) - r_0(\bX_i)} \abs{ \projr - \barr }\abs{\barr - \wh{r}(\bX_i)} = O_p(\epsilon_N^2 \delta_N), \nn  \\ 
& \aveiN \abs{\wh{r}(\bX_i) - r_0(\bX_i)}^2 \abs{ \projr - \barr }  = O_p(\epsilon_N \delta_N^2). \nn 
\end{align}
By the uniform boundness of $\wh{r}$ and $r_0$,
$\norm{\wh{r} - r_0}_{L_2(P)} = O_p(\delta_N)$,
and \eqref{eq: max bar-hatr}, we have 
\begin{align}
    & \aveiN  \abs{\wh{r}(\bX_i) - r_0(\bX_i)} \abs{\barr - \wh{r}(\bX_i)}^2 = O_p(\epsilon_N^2) \nn \\ 
    & \aveiN  \abs{\wh{r}(\bX_i) - r_0(\bX_i)}^2 \abs{\barr - \wh{r}(\bX_i)} =
 O_p(\epsilon_N\delta_N^2 ), \nn 
\end{align}
where the second result is obtained from the Cauchy-Schwarz inequality. 
Collecting the above results and plugging them into \eqref{eq: D2N-1}, 
we can bound $|D_{2,N}|$ by 
\begin{align}
    |D_{2,N}| & \leq O_p(\epsilon_N^2 \delta_N^2) + O_p(\epsilon_N \delta_N^2) +O_p(\epsilon_N \delta_N^2) + O_p(\epsilon_N^2) \nn \\  & = o_p\left( \frac{\epsilon_N}{\sqrt{N}}\right),
\end{align}
where the equality is due to $\epsilon_N = o(N^{-\frac{1}{2}})$ and $\delta_N = o_p(N^{-\frac{1}{4}})$.  

To sum up, we have shown that $$E_{3,N} = D_{1, N} + D_{2, N} = o_p\left( \frac{\epsilon_N}{\sqrt{N}}\right),$$
which together with the result for $E_{1,N} + E_{2,N}$ in \eqref{eq: E1+E2} yield 
\begin{align}
    & \frac{1}{N} \sumiN \left\{e(\delta_i, \bX_i; \projr - r_0) - e(\delta_i, \bX_i; \wh{r} - r_0)   \right\} \nn \\
=&  \epsilon_N(1- \epsilon_N) \E \left( \frac{1-\delta}{1-p} \{\wh{r}(\bX_i)- r_0(\bX) \}m_{\bv}(\bX_i)\right) + o_p\left(\frac{\epsilon_N}{\sqrt{N}} \right), \nn 
\end{align}
which is the desired result.

%%%%%%%%%%%%%%%%%%%%%%%%%%%%%%%%%%%%%%%%%%%%%%%%%%%%%%%%%%%
\newpage

\section{ Additional simulation results}
\begin{table}[ht]
    \centering
\begin{tabular}{c c c c c c c c }
    \hline
    \hline 
    \multicolumn{6}{c}{ $p=1$ } \\
  \hline
  \hline
$n$ & DIM & KLIEP & KMM & RULSIF & RF \\ 
  \hline
  \multirow{2}{*}{$100$}& 0.50 & 3.22 & 12.77 & 8.90 & 58.45 \\ 
 & (0.39) & (3.48) & (6.43) & (14.67) & (3.11) \\ 
  \hline
  \multirow{2}{*}{$250$} &  0.40 & 2.69 & 5.36 & 3.50 & 58.74 \\ 
  &(0.31) & (3.44) & (3.25) & (5.08) & (2.07) \\ 
  \hline
  \multirow{2}{*}{$500$} &  0.37 & 2.41 & 2.59 & 1.52 & 58.39 \\ 
 & (0.23) & (0.9) & (1.28) & (0.83) & (1.21) \\ 
  \hline
  \multirow{2}{*}{$1000$} & 0.29 & 2.54 & 1.24 & 1.19 & 58.31 \\ 
 & (0.14) & (0.77) & (0.70) & (0.78) & (1.08) \\ 
  \hline
  \multirow{2}{*}{$1500$} & 0.27 & 2.36 & 0.85 & 0.89 & 58.55 \\ 
  & (0.13) & (0.48) & (0.40) & (0.44) & (0.86) \\ 
   \hline
    \hline 
    \multicolumn{6}{c}{ $p=5$ } \\
  \hline
  \hline
%  $n$ & DIM & KLIEP & KMM & RuLSIF & RF \\ 
%     \hline
  \multirow{2}{*}{$100$}& 3.99 & 17.68 & 322.39 & 10.46 & 56.69 \\ 
  & (1.19) & (84.65) & (58.14) & (6.99) & (3.94) \\ 
  \hline
  \multirow{2}{*}{$250$} &  3.17 & 9.28 & 237.59 & 7.49 & 56.35 \\ 
  & (0.89) & (2.67) & (49.94) & (2.36) & (2.39) \\ 
  \hline
  \multirow{2}{*}{$500$} &  2.69 & 9.71 & 129.12 & 7.25 & 56.58 \\ 
  & (0.87) & (2.22) & (26.78) & (0.7) & (1.88) \\     
  \hline
  \multirow{2}{*}{$1000$} &  2.01 & 9.82 & 63.52 & 7.15 & 56.43 \\ 
  & (0.54) & (1.75) & (8.87) & (0.48) & (1.23) \\ 
  \hline
  \multirow{2}{*}{$1500$} &  1.78 & 9.59 & 43.01 & 7.19 & 56.35 \\ 
 & (0.42) & (0.96) & (6.20) & (0.43) & (0.99) \\ 
 \hline
    \hline 
    \multicolumn{6}{c}{ $p=10$ } \\
  \hline
  \hline
  \multirow{2}{*}{$100$}&  10.82 & 19.98 & 243.34 & 17.84 & 63.06 \\ 
  & (3.07) & (8.48) & (36.84) & (8.55) & (6.81) \\ 
  \hline
  \multirow{2}{*}{$250$} & 8.50 & 20.57 & 261.77 & 16.47 & 62.70 \\ 
 & (1.96) & (17.93) & (23.23) & (5.72) & (3.86) \\ 
  \hline
  \multirow{2}{*}{$500$} &  6.27 & 22.35 & 281.34 & 15.59 & 62.55 \\ 
  & (1.66) & (39.05) & (21.68) & (1.36) & (2.83) \\ 
  \hline
  \multirow{2}{*}{$1000$} &  4.63 & 18.28 & 276.43 & 15.33 & 62.06 \\ 
  & (1.10) & (1.55) & (15.74) & (0.85) & (1.98) \\ 
  \hline
  \multirow{2}{*}{$1500$} & 3.92 & 18.41 & 254.6 & 15.59 & 62.50 \\ 
  & (0.83) & (1.31) & (15.33) & (0.88) & (1.54) \\ 
  \hline
  \hline 
  \multicolumn{6}{c}{ $p=15$ } \\
\hline
\hline
  \multirow{2}{*}{$100$}  & 18.17 & 28.31 & 203.27 & 25.95 & 71.36 \\ 
  & (4.69) & (8.08) & (24.18) & (6.07) & (9.54) \\ 
  \hline
  \multirow{2}{*}{$250$} & 14.23 & 28.23 & 210.66 & 24.61 & 70.83 \\ 
  & (3.64) & (7.19) & (18.70) & (3.52) & (6.30) \\ 
  \hline
  \multirow{2}{*}{$500$} &  9.94 & 28.04 & 223.85 & 24.15 & 69.79 \\ 
  & (2.48) & (6.09) & (14.72) & (2.32) & (4.21) \\ 
  \hline
  \multirow{2}{*}{$1000$} & 7.44 & 27.29 & 259.16 & 23.98 & 69.80 \\ 
  & (1.33) & (2.67) & (13.62) & (1.97) & (2.97) \\ 
  \hline
  \multirow{2}{*}{$1500$} & 
  6.48 & 27.21 & 251.76 & 24.14 & 69.92 \\ 
 & (0.97) & (1.87) & (11.58) & (1.11) & (1.99) \\ 
   \hline
\end{tabular}
\end{table}
